# Supplementary material for: Task-Based Effectiveness of Interactive Contiguous Area Cartograms
Source: arXiv:2011.09714 ancillary file (2020-11-19)
Supplement: Supplementary file 1 [file experiment_design_and_results.pdf]

# Online Supplemental Text: Experiment Design and Results

Task-Based Effectiveness of Interactive Contiguous Area Cartograms

Ian K. Duncan, Shi Tingsheng, Simon T. Perrault, and Michael T. Gastner

## 1 Order in which combinations of regions, task types, and interactive features appeared during the experiment

We use the abbreviations CSA (cartogram-switching animation only), IT (infotip only), and LB (linked brushing only).

| Qn | Region | Task type | Interactive feature | | | | |
|---|---|---|---|---|---|---|---|
| | | | participants 1, 6, . . . , 51 | participants 2, 7, . . . , 52 | participants 3, 8, . . . , 53 | participants 4, 9, . . . , 54 | participants 5, 10, . . ., 55 |
| 1 | Brazil | Cluster | All | None | LB | IT | CSA |
| 2 | Germany | Compare | IT | CSA | All | None | LB |
| 3 | Brazil | Detect Change | None | LB | IT | CSA | All |
| 4 | India | Recognize | IT | CSA | All | None | LB |
| 5 | Germany | Summarize | IT | CSA | All | None | LB |
| 6 | China | Detect Change | All | None | LB | IT | CSA |
| 7 | Germany | Filter | All | None | LB | IT | CSA |
| 8 | China | Compare | None | LB | IT | CSA | All |
| 9 | USA | Cluster | LB | IT | CSA | None | All |
| 10 | India | Filter | LB | IT | CSA | None | All |
| 11 | Brazil | Find Adjacency | None | LB | IT | CSA | All |
| 12 | USA | Find Top | All | None | LB | IT | CSA |
| 13 | China | Cluster | CSA | All | None | LB | IT |
| 14 | USA | Compare | CSA | All | None | LB | IT |
| 15 | China | Find Top | LB | IT | CSA | None | All |
| 16 | Germany | Find Adjacency | LB | IT | CSA | None | All |
| 17 | Brazil | Compare | LB | IT | CSA | None | All |
| 18 | China | Summarize | None | LB | IT | CSA | All |
| 19 | Brazil | Recognize | All | None | LB | IT | CSA |
| 20 | Germany | Find Top | CSA | All | None | LB | IT |
| 21 | India | Cluster | IT | CSA | All | None | LB |
| 22 | USA | Summarize | CSA | All | None | LB | IT |
| 23 | India | Find Adjacency | CSA | All | None | LB | IT |
| 24 | USA | Recognize | LB | IT | CSA | None | All |
| 25 | India | Summarize | All | None | LB | IT | CSA |
| 26 | China | Recognize | CSA | All | None | LB | IT |
| 27 | Brazil | Find Top | IT | CSA | All | None | LB |
| 28 | USA | Detect Change | IT | CSA | All | None | LB |
| 29 | Germany | Cluster | None | LB | IT | CSA | All |
| 30 | India | Compare | All | None | LB | IT | CSA |
| 31 | USA | Filter | None | LB | IT | CSA | All |
| 32 | Germany | Detect Change | LB | IT | CSA | All | None |
| 33 | India | Find Top | None | LB | IT | CSA | All |
| 34 | Brazil | Summarize | LB | IT | CSA | All | None |
| 35 | China | Filter | IT | CSA | All | None | LB |
| 36 | USA | Find Adjacency | IT | CSA | All | None | LB |
| 37 | Germany | Recognize | None | LB | IT | CSA | All |
| 38 | China | Find Adjacency | All | None | LB | IT | CSA |
| 39 | India | Detect Change | CSA | All | None | LB | IT |
| 40 | Brazil | Filter | CSA | All | None | LB | IT |

# 2 Error rates

Figure 1 shows the distribution of the total number of errors by participant during all 40 cartogram reading tasks. The distribution is roughly symmetric with a mean of 5.5 and a standard deviation of 2.3. The minimum is 0, the median is 5, and the maximum is 10. The interquartile range is 3. Because there are no outliers, we included all participants in the data analysis.

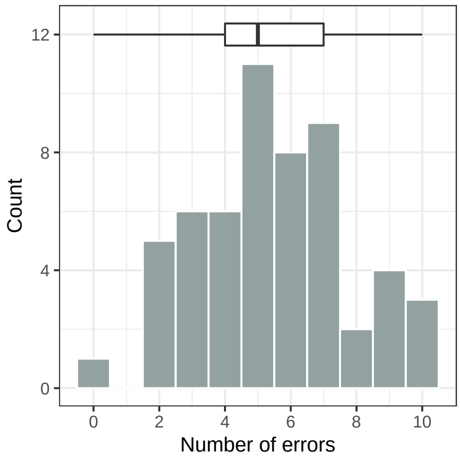


*Figure 1: Histogram and box plot of errors committed by participants during 40 cartogram reading tasks.*

The table below shows the error rates for different combinations of interactive features and task types. The last column indicates the $p$-value of the main effect. Bold font indicates a $p$-value below 0.05. For *Summarize* tasks, we report three results corresponding to three different values of $\theta$, defined as the largest relative change of areas between two cartograms for which we treat "Approximately no change" as a correct answer (see Sections 3.5 and 4.2 in the main text). If the post-hoc McNemar test identifies two conditions as being significantly different, we label both error rates with the same superscript.

| Task type | No interactivity | Cartogram-switching animation only | Linked brushing only | Infotip only | All features | Mean | $p$-value |
|---|---|---|---|---|---|---|---|
| Cluster | 12.7% | $30.9\%^{\alpha}$ | 18.2% | 9.1% | $5.5\%^{\alpha}$ | 15.3% | $< \mathbf{0.01}$ |
| Compare | 7.3% | 12.7% | $20.0\%^{\beta}$ | 5.5% | $1.8\%^{\beta}$ | 9.5% | **0.01** |
| Detect Change | 10.9% | 5.5% | 10.9% | 7.3% | 10.9% | 9.1% | 0.76 |
| Filter | 10.9% | 23.6% | $29.1\%^{\gamma}$ | 10.9% | $7.3\%^{\gamma}$ | 16.4% | $< \mathbf{0.01}$ |
| Find Adjacency | 3.6% | 0% | 3.6% | 5.5% | 3.6% | 3.3% | 0.62 |
| Find Top | 5.5% | 1.8% | 0% | 1.8% | 1.8% | 2.2% | 0.41 |
| Recognize | 0% | 0% | 0% | 0% | 0% | 0% | – |
| Summarize ($\theta = 0.5\%$) | $85.5\%^{\delta,\epsilon}$ | $41.8\%^{\delta,\zeta,\eta}$ | $87.3\%^{\zeta,\vartheta}$ | $81.8\%^{\eta,\iota}$ | $45.5\%^{\epsilon,\vartheta,\iota}$ | 68.4% | $< \mathbf{10^{-9}}$ |
| Summarize ($\theta = 1.0\%$) | $74.5\%^{\kappa,\lambda}$ | $23.6\%^{\kappa,\mu,\nu}$ | $70.9\%^{\mu,\xi}$ | $70.9\%^{\nu,o}$ | $27.3\%^{\lambda,\xi,o}$ | 53.5% | $< \mathbf{10^{-11}}$ |
| Summarize ($\theta = 2.0\%$) | $47.3\%^{\pi,\rho}$ | $16.4\%^{\pi,\sigma,\tau}$ | $45.5\%^{\sigma,\upsilon}$ | $50.9\%^{\tau,\phi}$ | $12.7\%^{\rho,\upsilon,\phi}$ | 34.5% | $< \mathbf{10^{-6}}$ |

The table reveals that error rates for *Summarize* tasks were significantly reduced in conditions that included cartogram-switching animations, either as the only available feature or in combination with the other two features. In Fig. 2, we split the error rates for $\theta = 1.0\%$ by the task category (panoptic vs. elementary), the availability of cartogram-switching animations, and the self-assessment of participants prior to the experiment. The bar chart in Fig. 2a shows that participants who rated themselves as being familiar with interactive computer graphics ($\geq 4$ on a 5-point Likert scale) committed fewer errors when animations were available. Their error rate dropped from 83.3% (95% CI: $[68.6\%, 93.0\%]$)) to 32.1% (95% CI: $[15.9\%, 52.4\%]$). The error rates for participants who declared less familiarity with interactive computer graphics were 68.3% (95% CI: $[59.3\%, 76.4\%]$) without animations and 23.2% (95% CI: $[14.6\%, 33.8\%]$) with animations. We conclude that the error rates did not differ significantly between both groups of participants.

A similar picture emerges when we split participants by their reported tendency to look up unfamiliar locations on a map (Fig. 2b). Participants who rated themselves highly ($\geq 4$) on a 5-point Likert scale had an error rate of 59.6% (95% CI: $[45.8\%, 72.4\%]$) in *Summarize* tasks without animations and 26.3% (95% CI: $[13.4\%, 43.1\%]$)

with animations. Participants who rated themselves lower on the Likert scale had an error rate of 78.7% (95% CI: [69.8%, 86.0%]) without animations and 25.0% (95% CI: [15.5%, 36.6%]) with animations.

Unlike in *Summarize* tasks, we did not find any evidence that animations influenced the error rates in elementary tasks, regardless of whether the participants considered themselves to be familiar with interactive computer graphics (Fig. 2c) or whether they reported a strong tendency towards looking up unfamiliar locations on a map (Fig. 2d).

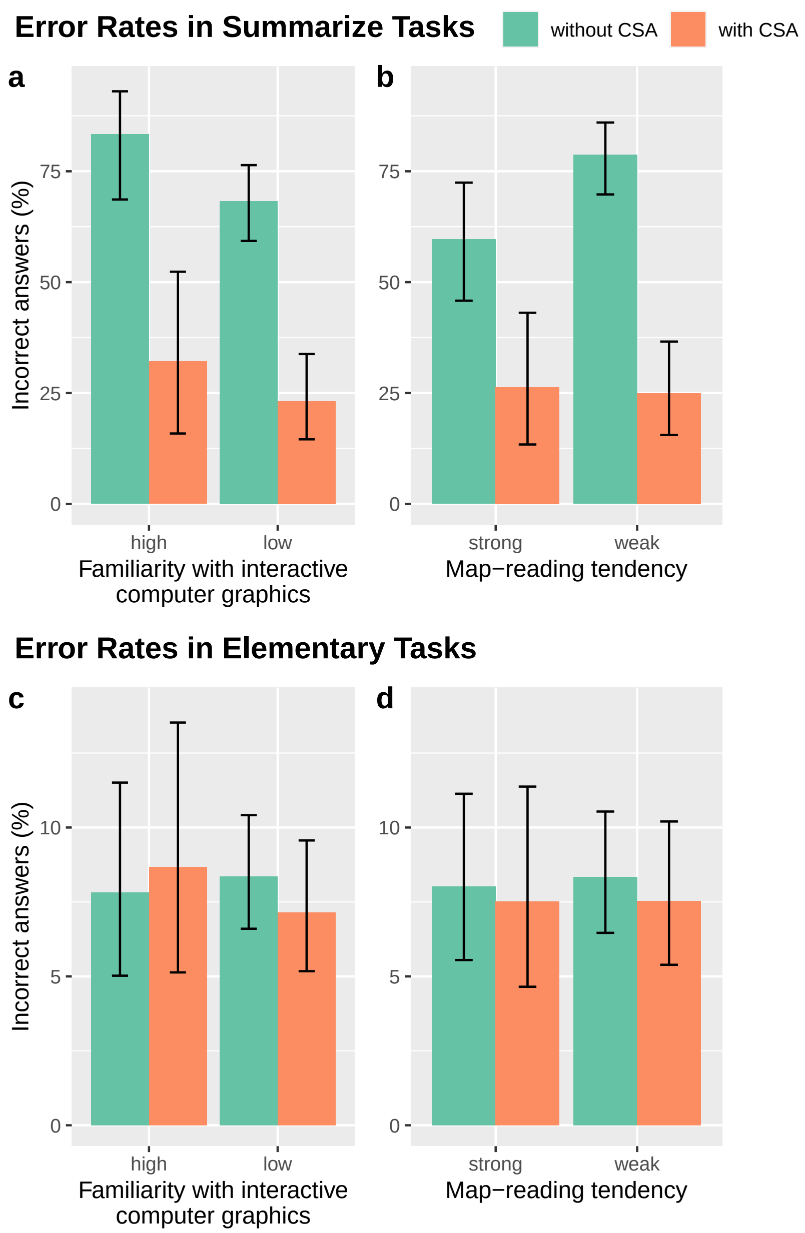


*Figure 2: Error rates by task category, availability of a cartogram switching animation (CSA), and the participants' self-assessment of their familiarity with interactive computer graphics and their tendency to read maps when they encounter the names of unfamiliar locations. Error bars correspond to 95% confidence intervals. Panels (a) and (b) show the results for the only panoptic task (Summarize) in our experiment. Panels (c) and (d) present the combined results for all other (i.e., elementary) tasks.*

## 3 Average response times

In the table below, the numbers in each cell are the mean and median response times in seconds for each correctly performed task. The first five columns show the performance for different combinations of interactive features and task types. The last column indicates the $p$-value of the main effect. Bold font indicates a $p$-value below 0.05. For *Summarize* tasks, we report three results corresponding to three different values of $\theta$, defined as the largest relative change of areas between two cartograms for which we treat "Approximately no change" as a correct answer (see Sections 3.5 and 4.2 in the main text). If the post-hoc Mann-Whitney U test identifies two conditions as being significantly different, we label both error rates with the same superscript. For *Summarize* with an area error threshold of $\theta = 0.5\%$, the Kruskal-Wallis test indicates a significant main effect ($p$-value 0.03), but none of the post-hoc tests identifies a significant difference between any pair of interactive-feature conditions.

| Task type | No interactivity | Cartogram-switching animation only | Linked brushing only | Infotip only | All features | Overall (mean, median) | $p$-value |
|---|---|---|---|---|---|---|---|
| Cluster | (59.4, 58.1) | (64.3, 52.7) | (65.4, 62.0) | (54.4, 52.6) | (60.7, 59.0) | (60.9, 56.9) | 0.61 |
| Compare | (32.7, 31.1) | (36.4, 35.5) | (31.4, 30.4) | $(39.6, 36.9)^{\chi}$ | $(31.5, 28.1)^{\chi}$ | (34.3, 32.2) | < **0.01** |
| Detect Change | (28.6, 25.4) | (28.4, 27.5) | $(26.2, 23.7)^{\psi,\omega}$ | $(33.7, 32.2)^{\psi}$ | $(33.1, 32.1)^{\omega}$ | (30.0, 28.2) | < **0.01** |
| Filter | (51.1, 45.2) | (50.4, 50.6) | (50.1, 47.3) | (58.0, 59.0) | (55.9, 50.0) | (53.1, 50.5) | 0.16 |
| Find Adjacency | (22.8, 21.3) | (25.1, 22.2) | (25.0, 23.0) | (23.1, 22.4) | (22.7, 20.2) | (23.7, 21.5) | 0.45 |
| Find Top | (22.3, 16.7) | (26.8, 22.3) | (29.0, 24.4) | (26.6, 20.2) | (29.9, 22.5) | (26.9, 20.5) | 0.22 |
| Recognize | (13.2, 11.4) | (13.4, 10.4) | (11.9, 9.9) | (11.9, 9.1) | (10.8, 10.0) | (12.3, 10.0) | 0.06 |
| ($\theta = 0.5\%$) | (43.8, 29.2) | (38.5, 40.2) | (29.2, 30.4) | (62.4, 57.9) | (43.1, 41.2) | (42.6, 40.0) | 0.03 |
| Summarize ($\theta = 1.0\%$) | (36.9, 29.2) | (38.4, 38.5) | (35.4, 34.4) | (48.5, 34.1) | (39.1, 34.5) | (39.3, 34.1) | 0.49 |
| ($\theta = 2.0\%$) | (40.2, 33.6) | (38.0, 36.7) | (41.2, 42.2) | (47.8, 42.9) | (39.9, 35.8) | (40.9, 36.1) | 0.68 |

## 4 Mean user ratings

In the first seven rows and columns 2–4 of the table below, each cell shows the mean user ratings for a combination of a phrase pair in the attitude study conducted at the end of our experiment. Responses were on a 5-point Likert scale, where 1 was the most negative and 5 the most positive response. The bottom row contains the average over each interactive feature. The rightmost column shows the average over each phrase pair.

| Phrase pair | Cartogram-switching animation | Linked brushing | Infotip | Mean |
|---|---|---|---|---|
| Difficult to use – Easy to use | 4.53 | 4.60 | 4.65 | 4.59 |
| Hindering – Helpful | 4.16 | 4.55 | 4.42 | 4.38 |
| Redundant – Informative | 4.13 | 4.33 | 4.49 | 4.32 |
| Forms immediate impression: yes – no | 4.07 | 4.38 | 3.89 | 4.12 |
| Ugly – Elegant | 3.91 | 4.24 | 3.76 | 3.97 |
| Boring – Entertaining | 4.00 | 3.96 | 3.45 | 3.81 |
| Conventional – Innovative | 3.71 | 3.78 | 2.96 | 3.48 |
| Mean | 4.07 | 4.26 | 3.95 | |

# 5 Distribution of ratings

Each bar chart in Fig. 3 shows the distribution of responses for the pair of phrases printed at the top of the chart.

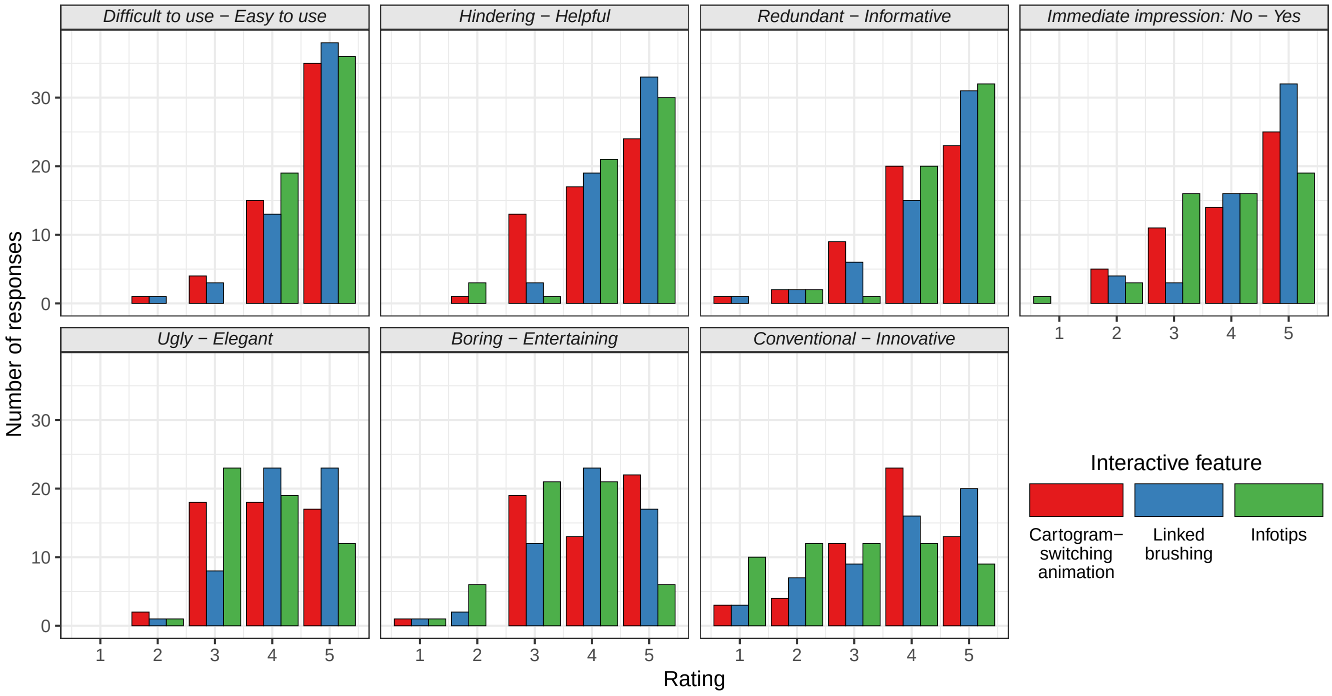


*Figure 3: Responses given during the attitude study.*

# 6 Performance comparison of different countries shown on the cartograms

In Fig. 4, we show the error rates (left) and response times (right) of all trials grouped by country and aggregated over all task types. Error bars indicate 95% confidence intervals. Brackets indicate statistically significant differences between pairs of countries at a significance level of 0.05. The asterisks above the brackets indicate $p$-values ($*$: $\leq 0.05$, $**$: $\leq 0.01$, $***$: $\leq 0.001$, $****$: $\leq 0.0001$).

According to a proportion test, the country had no significant effect on the error rate [$\chi^2(4) = 4.48$, $p = 0.35$]. However, a Kruskal-Wallis test identifies a significant effect on the response time [$\chi^2(4) = 48.19$, $p < 10^{-9}$]. The slowest response times were for Brazil (mean 38.4 s, median 33.9 s) followed by mainland China and Taiwan (mean 36.5 s, median 33.2 s). The fastest response times occurred for the United States (mean 29.4 s, median 23.2 s). A post-hoc Mann Whitney U test with Bonferroni-Holm correction results in a 95% confidence interval $[4.3\,\mathrm{s}, 11.8\,\mathrm{s}]$ for the pseudomedian difference between Brazil and the United States. When comparing mainland China and Taiwan to the United States, the 95% confidence interval is $[3.4\,\mathrm{s}, 11.1\,\mathrm{s}]$.

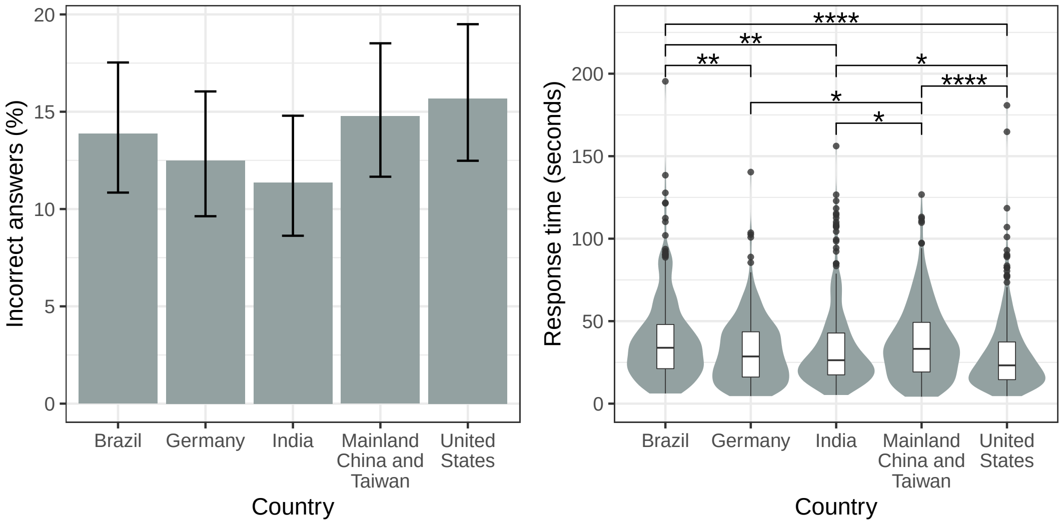


*Figure 4: Performance by country.*

In Fig. 5, we show the median response time as a function of the number of administrative units on the map. The line and confidence bands are the results of least-squares regression. The slope of the regression line is not significantly different from zero ($-0.20$ with a 95% confidence interval $[-0.78, 0.38]$). Hence, our data do not provide evidence that the number of administrative units has an influence on the performance in cartogram reading tasks.

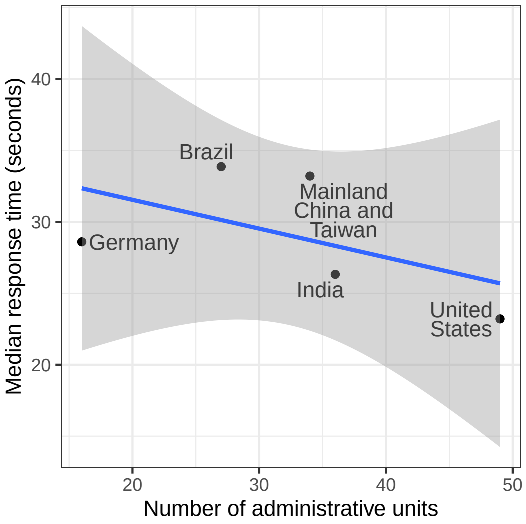


*Figure 5: Linear regression does not reveal a dependence of the median response time on the number of administrative units on the map. The 95% confidence band is shown in gray.*

## 7 Percentage of tasks in which an animation was used if available

Because we adopted an objective-based task taxonomy, participants were free to choose whether they used an available interactive feature. In Fig. 6, we show the percentage of tasks in which users triggered a cartogram-switching animation if it was available (i.e., in the animation-only and all-features conditions). In *Summarize* tasks, every available animation was used because it was the only way to view both cartograms referred to in the question. For the same reason, participants also would have had to play the animation in *Detect Change* tasks, and in 95.4% of the cases they indeed followed the instruction: "you may have to use the cartogram selector tab to view both cartograms." Judging from the screen recordings of the other cases, some participants apparently thought that the *Detect Change* task was to compare the equal-area map with the cartogram that was visible at the start of the task, so the animation may not have appeared to be necessary. For all other task types, animation use was below 20%. For this reason, it was unlikely that animations caused any performance change in these cases. Apart from *Summarize* and *Detect Change* tasks, nominally significant differences were likely due to randomness rather than the availability of animations.

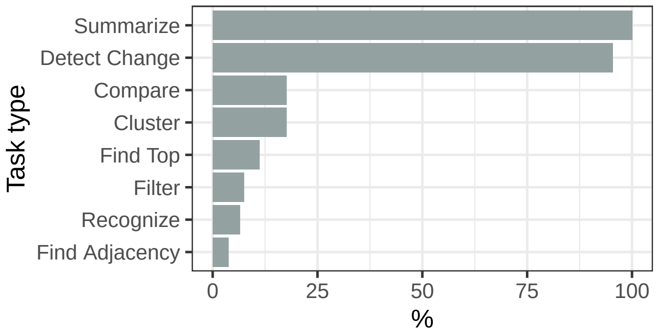


*Figure 6: Percentage of tasks in which a cartogram-switching animation was used if available.*
