# Supplementary material for: Task-Based Effectiveness of Interactive Contiguous Area Cartograms
Source: arXiv:2011.09714 ancillary file (2020-11-19)
Supplement: Supplementary file 2 [file questionnaire.pdf]

# Questionnaire

Ian K. Duncan, Shi Tingsheng, Simon T. Perrault, Michael T. Gastner

December 20, 2019

# Introduction

This document contains the questions that participants answered during the experiment. The experiment is broken up into four sections:

1. Preliminary questions
2. Color vision test
3. Cartogram analysis questions
4. Attitude test

For each question in the cartogram analysis section, the following information is given:

1. A screenshot of the cartogram viewing interface shown to participants during the experiment, with all interactive features enabled.
2. Question task type from our task taxonomy. This was not shown to participants during the experiment.
3. The text of the question.
4. The multiple choice answer options. Most questions have only one correct answer. Questions with multiple correct answers will be indicated with instructions in the question text.

## Preliminary Questions

1. How old are you?

---

2. What is your gender?

A. Male

B. Female

C. Other

D. Prefer not to say

3. What is your highest level of education?

A. High School graduate

B. Some college

C. Associate's and/or Bachelor's degree

D. Bachelor's degree

E. Master's degree

F. Doctorate or Professional degree

4. How familiar are you with interactive computer graphics?

A. 1: Very unfamiliar

B. 2: Unfamiliar

C. 3: Somewhat familiar

D. 4: Familiar

E. 5: Very familiar

5. How familiar are you with cartograms?

A. 1: Very unfamiliar

B. 2 :Unfamiliar

C. 3: Somewhat familiar

D. 4: Familiar

E. 5: Very familiar



6.

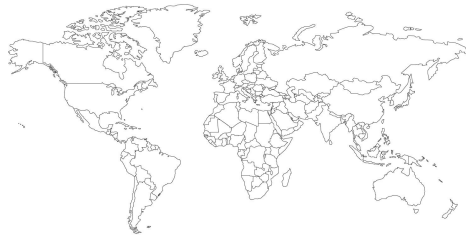

Consider the world map above. Would you be able to point at the location where you were born?

A. 1: Yes, with confidence.

B. 2: Yes, with a little effort.

C. 3: Yes, with much effort.

D. 4: Possibly, but I'm uncertain.

E. 5: No.

7. When you encounter the names of unfamiliar locations (e.g. countries, islands, lakes), how frequently do you immediately look them up on a map to find out where they are?

A. 1: Never

B. 2: Rarely

C. 3: Sometimes

D. 4: Generally

E. 5: Always

## Vision Test Questions

1. Please enter the number displayed in the image below. If you do not see any number, please enter "NA."

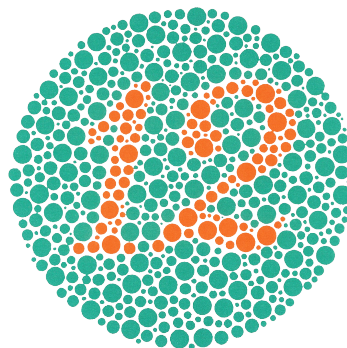

---

2. Please enter the number displayed in the image below. If you do not see any number, please enter “NA.”

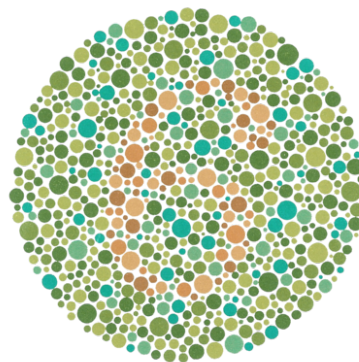

---

3. Please enter the number displayed in the image below. If you do not see any number, please enter "NA."

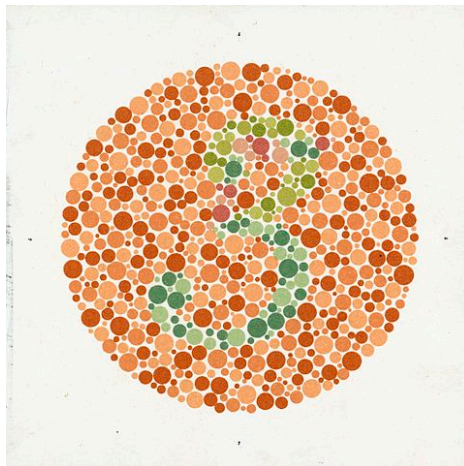

---

4. Please enter the number displayed in the image below. If you do not see any number, please enter "NA."

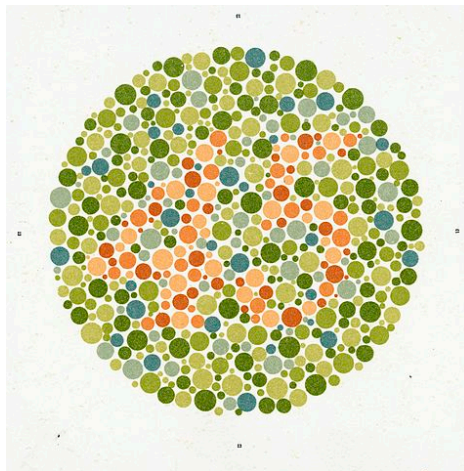

---

5. Please enter the number displayed in the image below. If you do not see any number, please enter "NA."

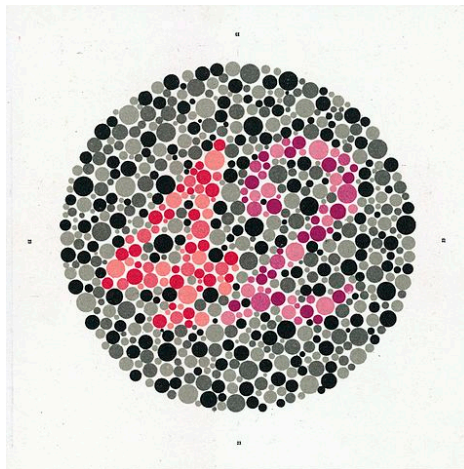

---

6. Please enter the number displayed in the image below. If you do not see any, please enter "NA."

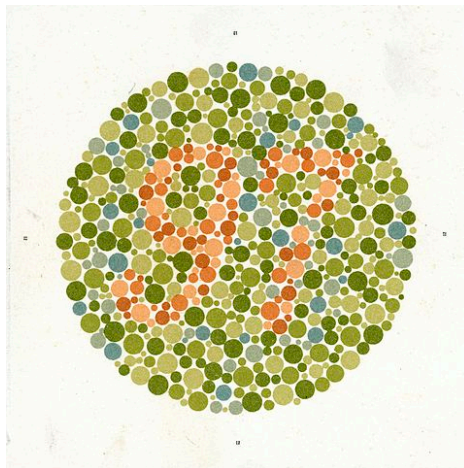

---



# Multiple Choice Questions

## Question 1

You have access to the infotips, parallel highlighting, and map switching features.

Hover over map regions to see more information.

Population Land Area

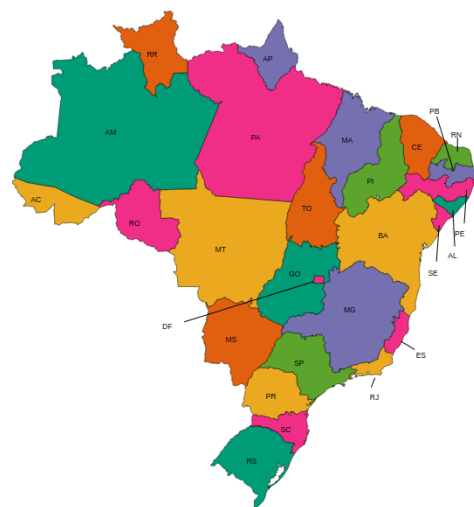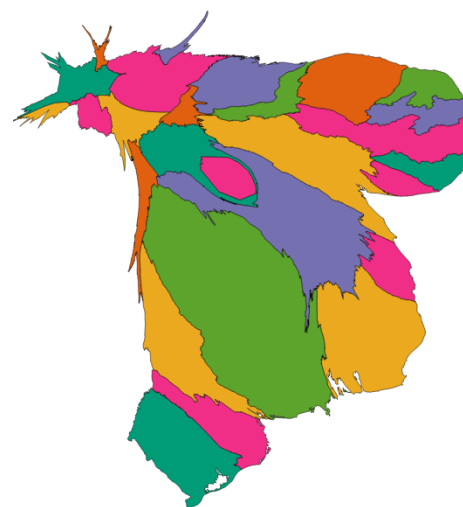

Next »

**(Cluster) Question 1 out of 43** On the other monitor, you can see a conventional map of Brazil (left) and a cattle population cartogram (right). Out of the states listed below, which has a cattle population most similar to Mato Grosso do Sul (MS)?

A. Rondonia (RO)

B. Para (PA)

C. Mato Grosso (MT)

D. Sao Paulo (SP)

## Question 2

You have access to the infotips, parallel highlighting, and map switching features.

Hover over map regions to see more information.

GDP Population Land Area

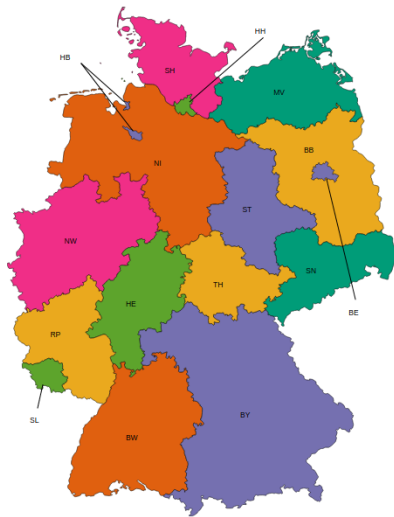

« Previous

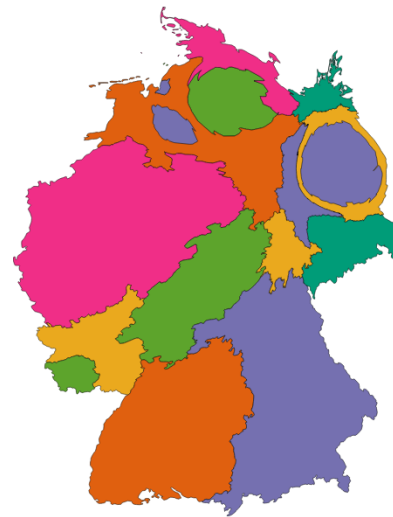

Next »

**(Compare) Question 2 out of 43** On the other monitor, you can see a conventional map of Germany (left) and a GDP cartogram (right). Is the GDP of Mecklenburg-Vorpommern (MV)

- higher than,
- approximately equal to or
- lower than

the GDP of Rheinland-Pfalz (RP)?

A. Higher

C. Lower

B. Approximately equal

### Question 3

You have access to the infotips, parallel highlighting, and map switching features.

Hover over map regions to see more information.

Cows Population Land Area

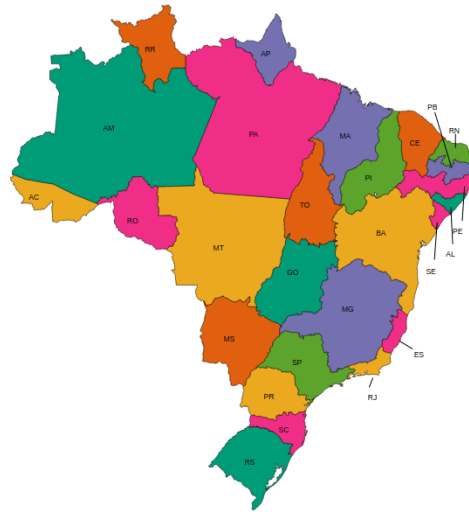

« Previous

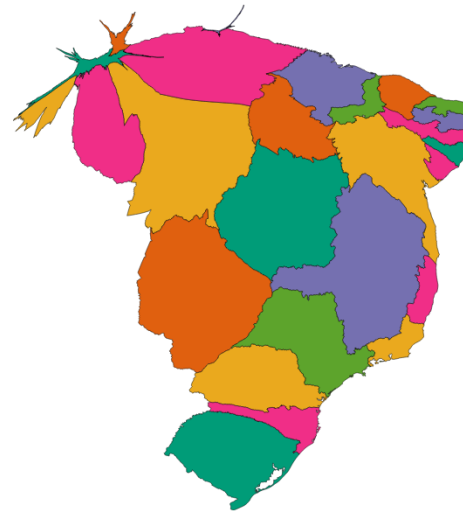

Next »

(Detect change) **Question 3 out of 43** On the other monitor, you can see a conventional map of Brazil (left), a cattle population cartogram and a human population cartogram (right). You may have to use the cartogram selector tab to view both cartograms. Is the area of Amazonas (AM) in the **cattle population cartogram**

- higher than,
- approximately equal to or
- lower than

its area in the **human population cartogram**?

A. Higher

C. Lower

B. Approximately equal

#### Question 4

You have access to the infotips, parallel highlighting, and map switching features.

Hover over map regions to see more information.

Population Land Area

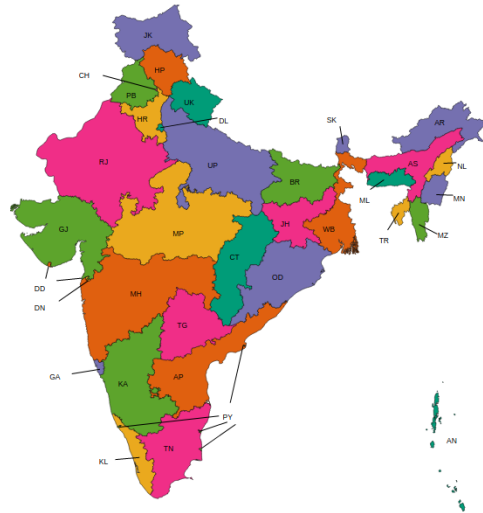

« Previous

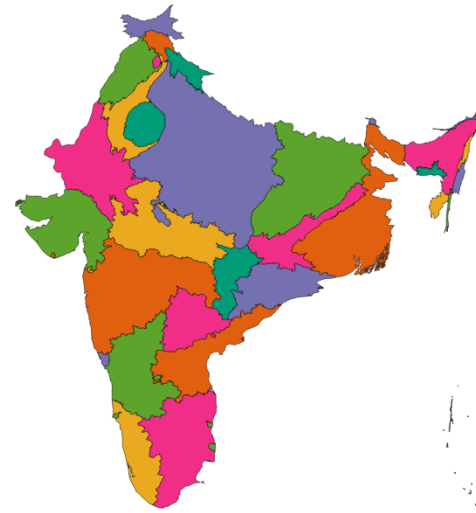

Next »

**(Recognize) Question 4 out of 43** On the other monitor, you can see a conventional map of India (left) and a population cartogram (right). What is the name of the state highlighted red in the population cartogram below?

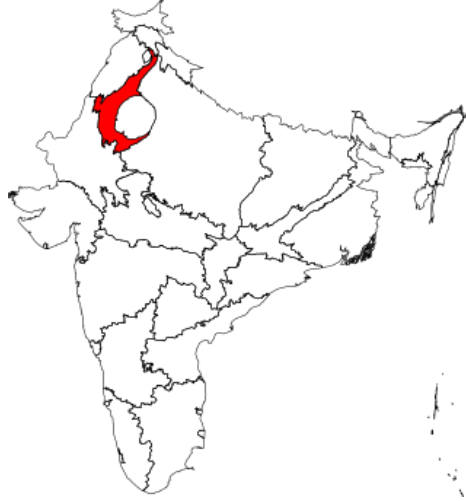

A. Haryana (HR)

B. Punjab (PB)

C. Rajasthan (RJ)

D. Himachal Pradesh (HP)

### Question 5

You have access to the infotips, parallel highlighting, and map switching features.

Hover over map regions to see more information.

Population (1985) Population (2015) Area

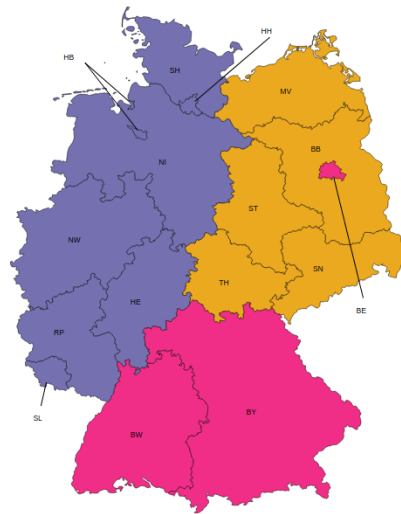

« Previous

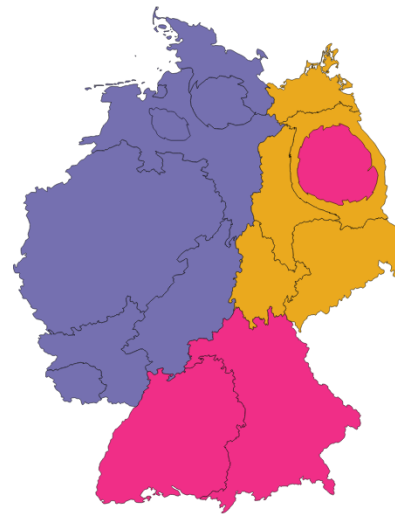

Next »

**(Summarize) Question 5 out of 43** On the other monitor, you can see a conventional map of Germany (left) and population cartograms for the years 1985 and 2015 (right). You may have to use the cartogram selector tab to view both cartograms. Three different regions are highlighted in yellow, purple and pink. What can you say about the change in population for each region from 1985 to 2015?

|                      |           |                            |              |
|----------------------|-----------|----------------------------|--------------|
| <b>Yellow Region</b> | A. Growth | B. Approximately No Change | C. Shrinking |
| <b>Pink Region</b>   | A. Growth | B. Approximately No Change | C. Shrinking |
| <b>Purple Region</b> | A. Growth | B. Approximately No Change | C. Shrinking |



### Question 6

You have access to the infotips, parallel highlighting, and map switching features.

Hover over map regions to see more information.

GDP Population Land Area

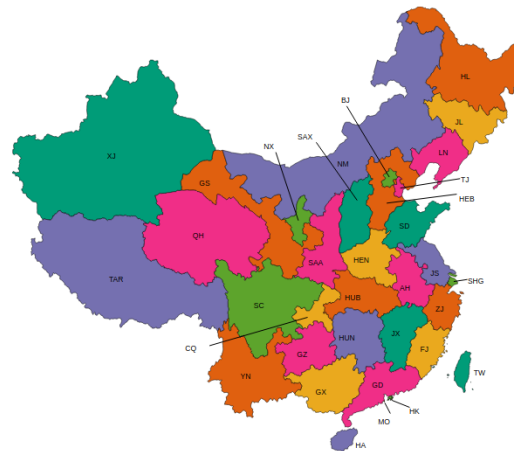

« Previous

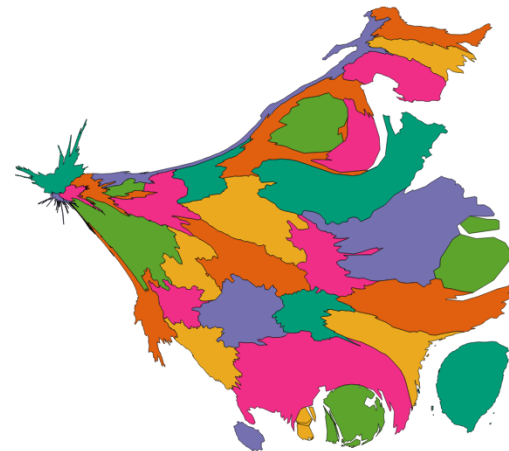

Next »

**(Detect change) Question 6 out of 43** On the other monitor, you can see a conventional map of Mainland China and Taiwan (left) and a GDP cartogram and a population cartogram (right). You may have to use the cartogram selector tab to view both cartograms. Is the area of Heilongjiang (HL) on the **GDP cartogram**

- higher than,
- approximately equal to or
- lower than

its area on the **population cartogram**?

A. Higher

C. Lower

B. Approximately equal

### Question 7

You have access to the infotips, parallel highlighting, and map switching features.

Hover over map regions to see more information.

Population Land Area

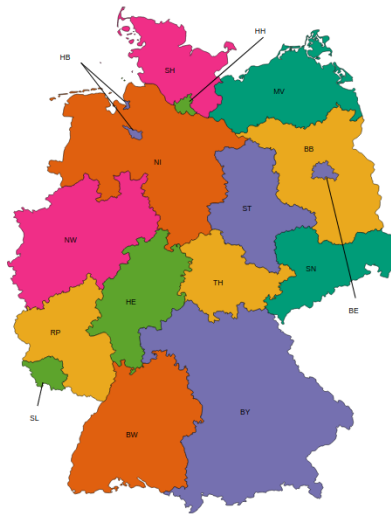

« Previous

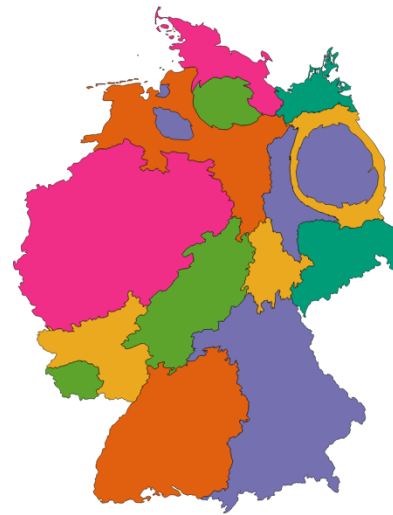

Next »

**(Filter) Question 7 out of 43** On the other monitor, you can see a conventional map of Germany (left) and a population cartogram (right). Out of the states listed below, which one(s) have a population higher than Baden-Wuerttemberg (BW)? **There may be more than one correct answer.**

- A. Nordrhein-Westfalen (NW)
- C. Niedersachsen (NI)

- B. Hessen (HE)
- D. Bayern (BY)

### Question 8

You have access to the infotips, parallel highlighting, and map switching features.

Hover over map regions to see more information.

GDP Population Land Area

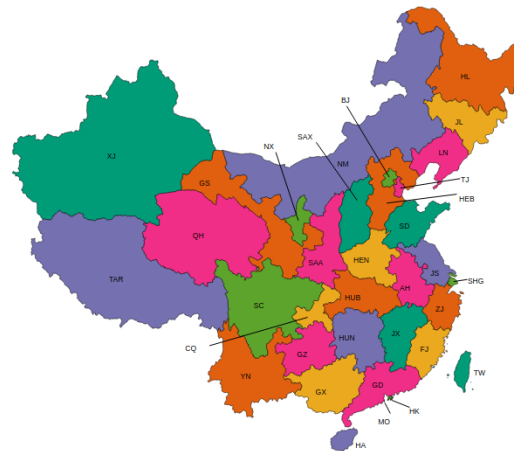

« Previous

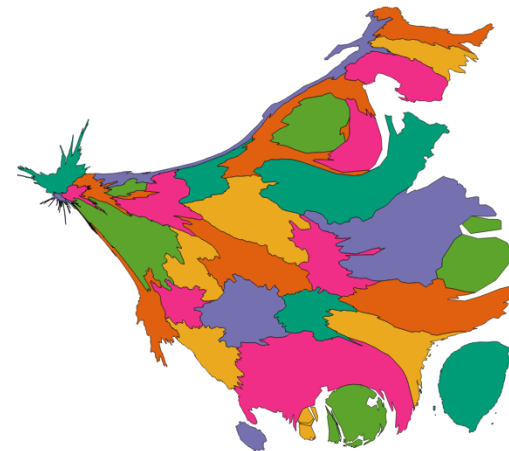

Next »

**(Compare) Question 8 out of 43** On the other monitor, you can see a conventional map of Mainland China and Taiwan (left) and a GDP cartogram (right). You may have to use the cartogram selector tab to view both cartograms. Is the GDP of Taiwan (TW)

- higher than,
- approximately equal to or
- lower than

the GDP of Zhejiang (ZJ)?

A. Higher

C. Lower

B. Approximately equal

### Question 9

You have access to the infotips, parallel highlighting, and map switching features.

Hover over map regions to see more information.

Crop Total (\$) Population Land Area

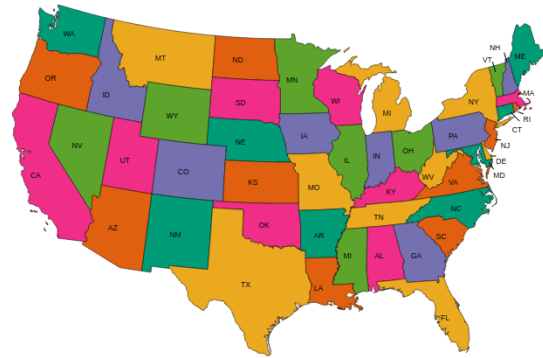

« Previous

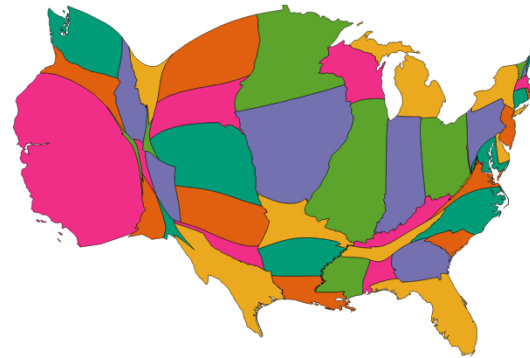

Next »

**(Cluster) Question 9 out of 43** On the other monitor, you can see a conventional map of the USA (left) and a crop production cartogram (right). Out of the states listed below, which has a crop production most similar to Minnesota (MN)?

A. Iowa (IA)

B. Illinois (IL)

C. California (CA)

D. Washington (WA)

### Question 10

You have access to the infotips, parallel highlighting, and map switching features.

Hover over map regions to see more information.

GDP Population Land Area

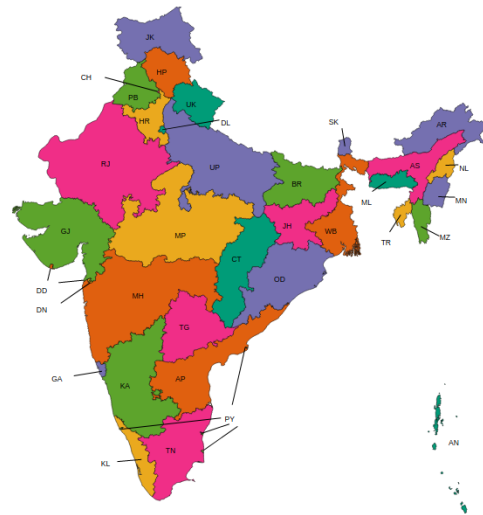

« Previous

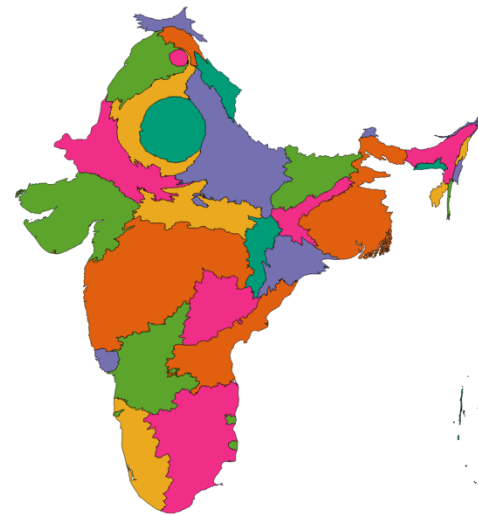

Next »

**(Filter) Question 10 out of 43** On the other monitor, you can see a conventional map of India (left) and a GDP cartogram (right). Out of the states listed below, which one(s) have a GDP higher than Delhi (DL)? **There may be more than one correct answer.**

- A. Arunachal Pradesh (AR)
- C. Puducherry (PY)

- B. Uttar Pradesh (UP)
- D. Punjab (PB)

### Question 11

You have access to the infotips, parallel highlighting, and map switching features.

Hover over map regions to see more information.

Population Land Area

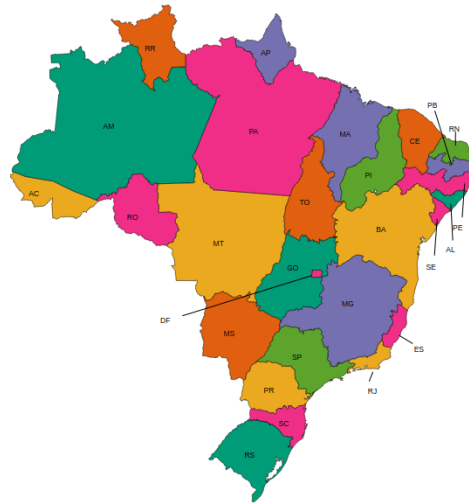

« Previous

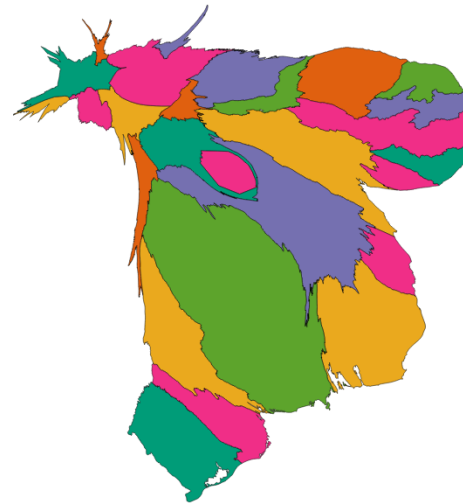

Next »

(Find adjacency) **Question 11 out of 43** On the other monitor, you can see a conventional map of Brazil (left) and a population cartogram (right). Which state(s) are **neighbours** of the state highlighted in red in the population cartogram below? **There may be more than one correct answer.**



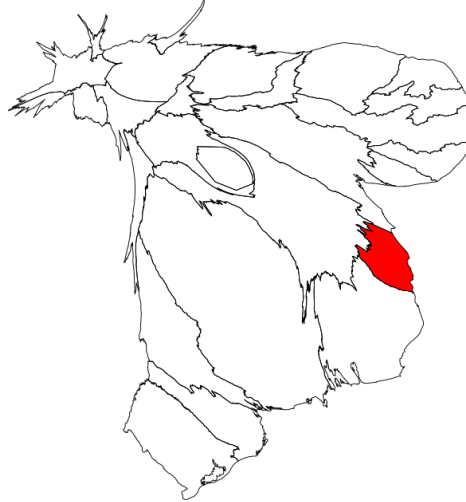

A. Bahia (BA)

B. Minas Gerais (MG)

C. Maranhao (MA)

D. Sergipe (SE)

### Question 12

You have access to the infotips, parallel highlighting, and map switching features.

Hover over map regions to see more information.

Crop Total (\$) Population Land Area

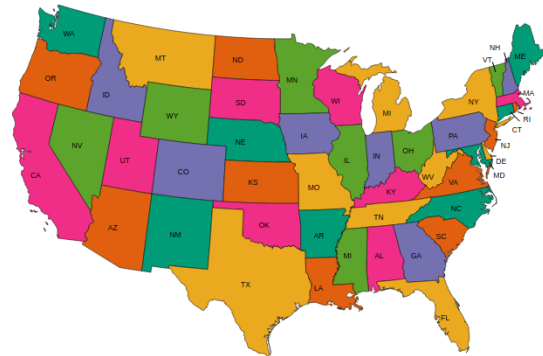

« Previous

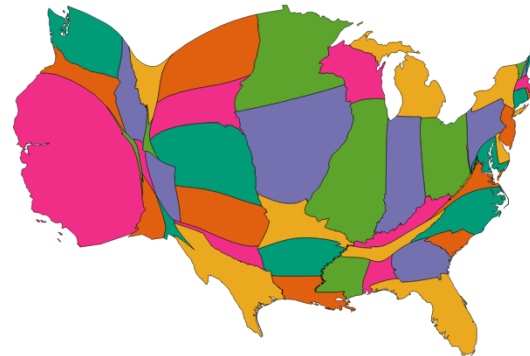

Next »

**(Find top-k) Question 12 out of 43** On the other monitor, you can see a conventional map of the USA (left) and a crop production cartogram (right). Which state of the USA has the highest crop production?

- A. California (CA)
- C. Maine (ME)

- B. Montana (MT)
- D. Iowa (IA)

### Question 13

You have access to the infotips, parallel highlighting, and map switching features.

Hover over map regions to see more information.

Population Land Area

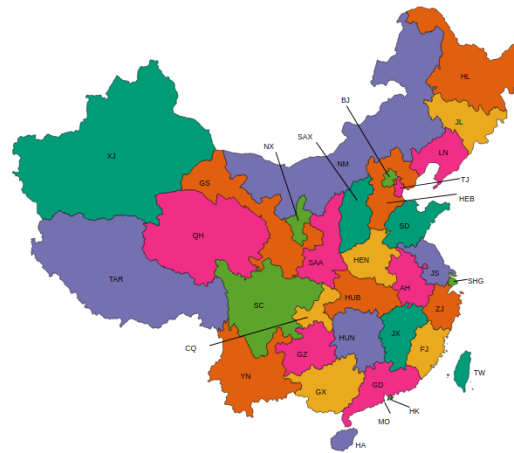

« Previous

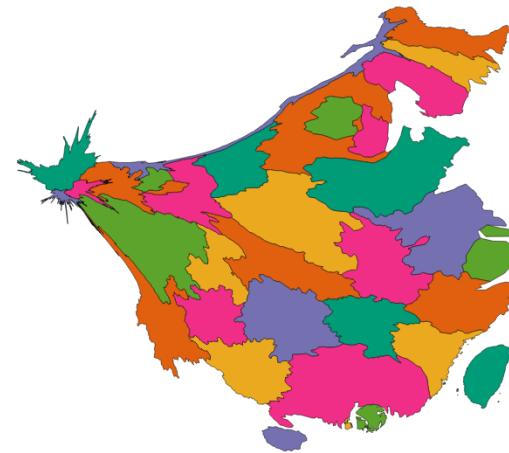

Next »

(Cluster) Question 13 out of 43 On the other monitor, you can see a conventional map of Mainland China and Taiwan (left) and a population cartogram (right). Out of the regions listed below, which has a population most similar to Hong Kong (HK)?

- A. Xinjiang (XJ)
- C. Yunnan (YN)

- B. Heilongjiang (HL)
- D. Ningxia (NX)

#### Question 14

You have access to the infotips, parallel highlighting, and map switching features.

Hover over map regions to see more information.

Electoral Votes Population Land Area

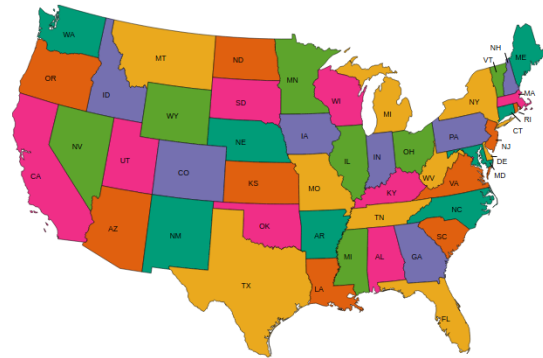

« Previous

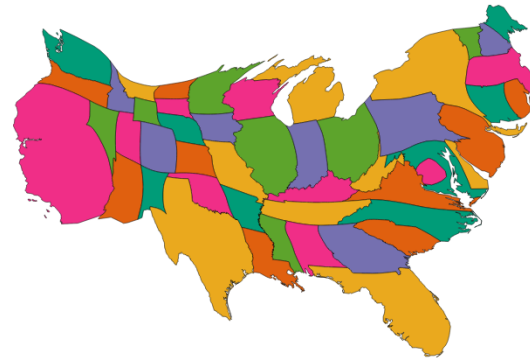

Next »

**(Compare) Question 14 out of 43** On the other monitor, you can see a conventional map of the USA (left) and an electoral vote cartogram (right). Does Maine (ME) have more, fewer or an approximately equal amount of electoral votes than New Hampshire (NH)?

A. More

B. Fewer

C. Approximately equal amount

### Question 15

You have access to the infotips, parallel highlighting, and map switching features.

Hover over map regions to see more information.

Population Land Area

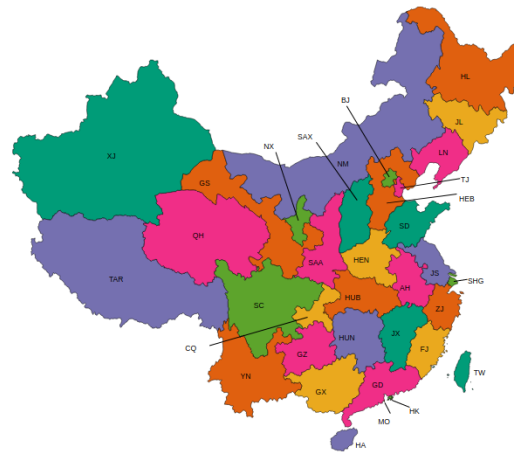

« Previous

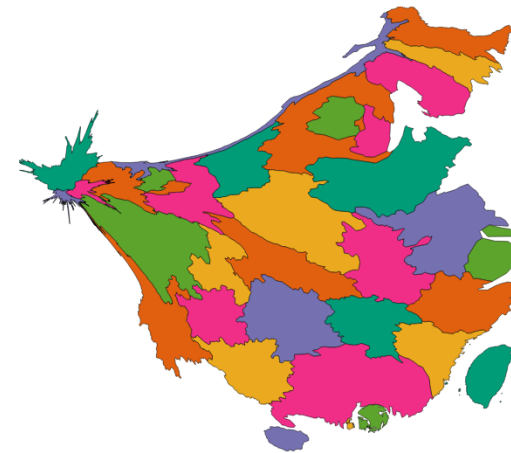

Next »

**(Find top-k)** Question 15 out of 43 On the other monitor, you can see a conventional map of Mainland China and Taiwan (left) and a population cartogram (right). Which region of China has the highest population?

- A. Guangdong (GD)
- C. Hong Kong (HK)

- B. Fujian (FJ)
- D. Beijing (BJ)

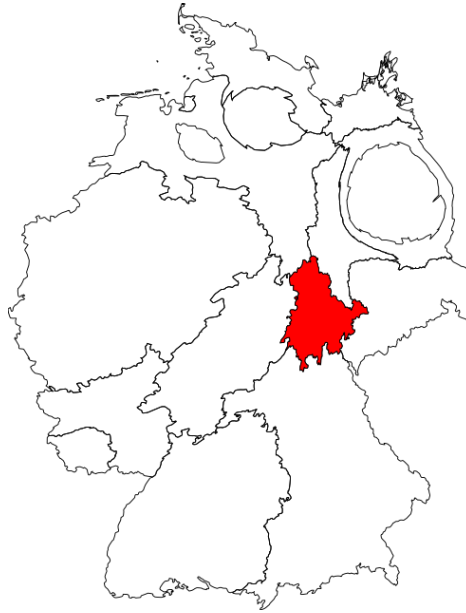

A. Berlin (BE)

B. Bayern (BY)

C. Saarland (SL)

D. Hessen (HE)

### Question 17

You have access to the infotips, parallel highlighting, and map switching features.

Hover over map regions to see more information.

GDP Population Land Area

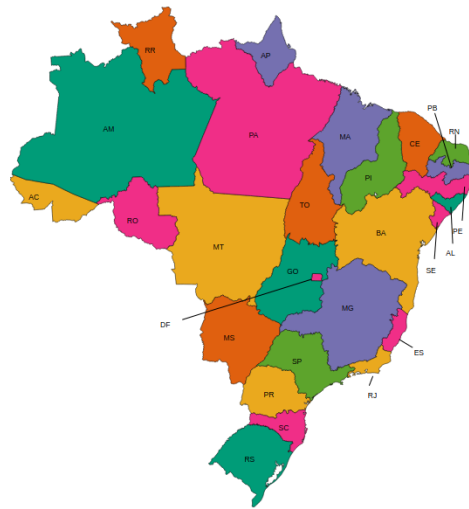

« Previous

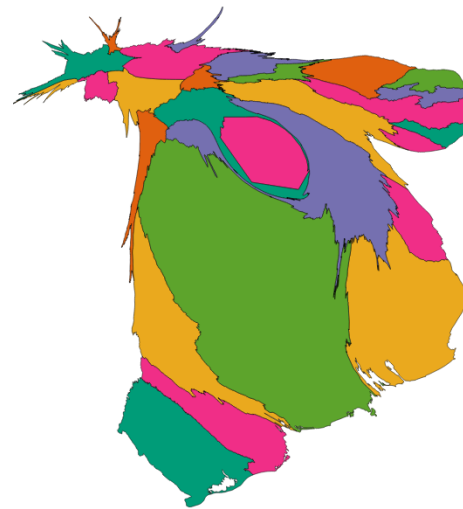

Next »

**(Compare) Question 17 out of 43** On the other monitor, you can see a conventional map of Brazil (left) and a GDP cartogram (right). Is the GDP of Rio de Janeiro (RJ)

- higher than,
- approximately equal to or
- lower than

the GDP of Rio Grande do Sul (RS)?

A. Higher

C. Lower

B. Approximately equal



### Question 18

You have access to the infotips, parallel highlighting, and map switching features.

Hover over map regions to see more information.

Population (2000) Population (2030) Area

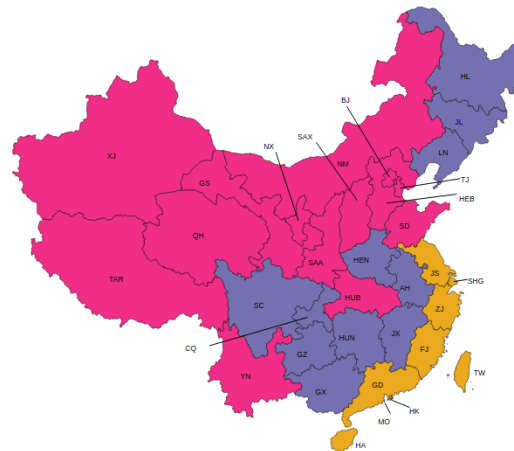

« Previous

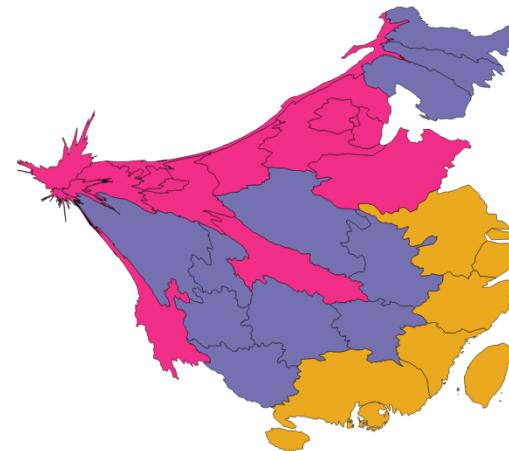

Next »

**(Summarize) Question 18 out of 43** On the other monitor, you can see a conventional map of Mainland China and Taiwan (left) and population cartograms for the years 2000 and 2030 (projected population, right). You may have to use the cartogram selector tab to view both cartograms. Three different regions are highlighted in yellow, purple and pink. What can you say about the projected change in population for each region from 2000 to 2030?

|                      |           |                            |              |
|----------------------|-----------|----------------------------|--------------|
| <b>Yellow Region</b> | A. Growth | B. Approximately No Change | C. Shrinking |
| <b>Pink Region</b>   | A. Growth | B. Approximately No Change | C. Shrinking |
| <b>Purple Region</b> | A. Growth | B. Approximately No Change | C. Shrinking |

### Question 19

You have access to the infotips, parallel highlighting, and map switching features.

Hover over map regions to see more information.

Population Land Area

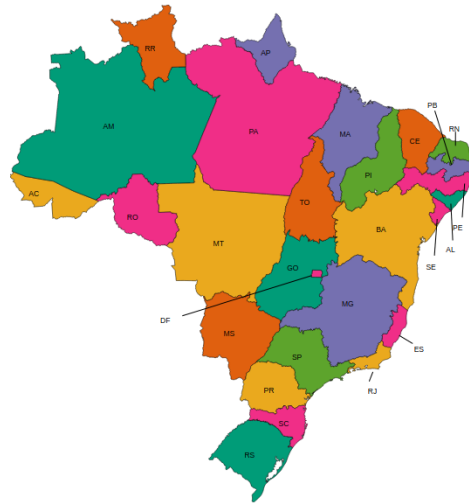

« Previous

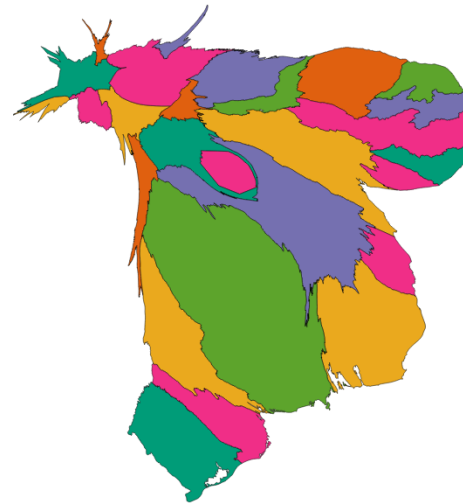

Next »

**(Recognize) Question 19 out of 43** On the other monitor, you can see a conventional map of Brazil (left) and a population cartogram (right). What is the name of the state highlighted in red in the population cartogram below?

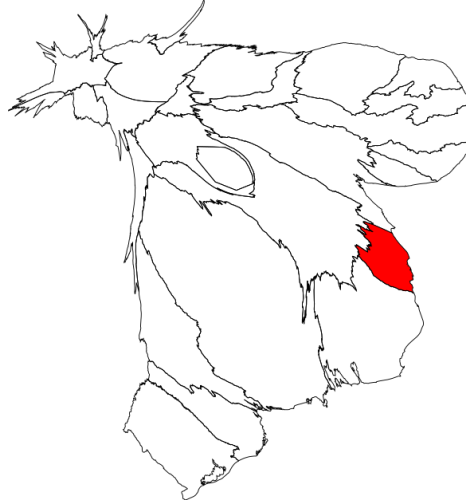

A. Espirito Santo (ES)

B. Sao Paulo (SP)

C. Amazonas (AM)

D. Rio Grande do Sul (RS)

### Question 20

You have access to the infotips, parallel highlighting, and map switching features.

Hover over map regions to see more information.

GDP Population Land Area

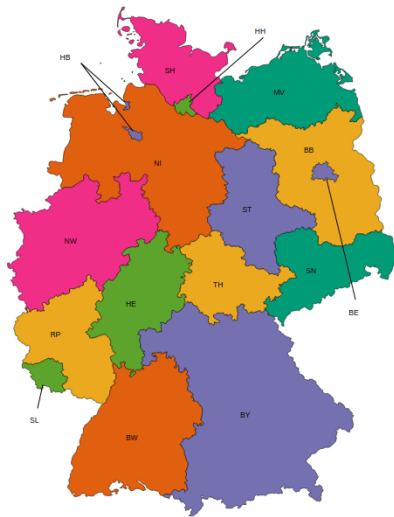

« Previous

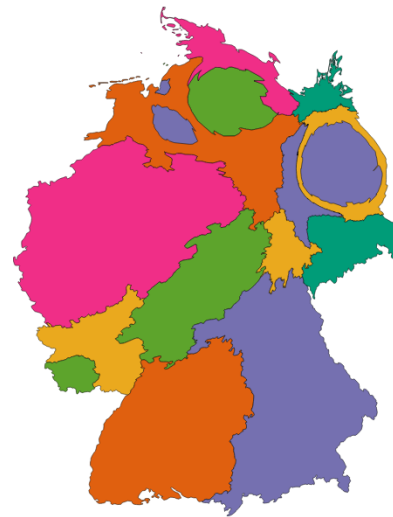

Next »

**(Find top-k) Question 20 out of 43** On the other monitor, you can see a conventional map of Germany (left) and a GDP cartogram (right). Which state of Germany has the highest GDP?

- A. Berlin (BE)
- B. Nordrhein-Westfalen (NW)
- C. Bremen (HB)
- D. Saarland (SL)

### Question 21

You have access to the infotips, parallel highlighting, and map switching features.

Hover over map regions to see more information.

GDP Population Land Area

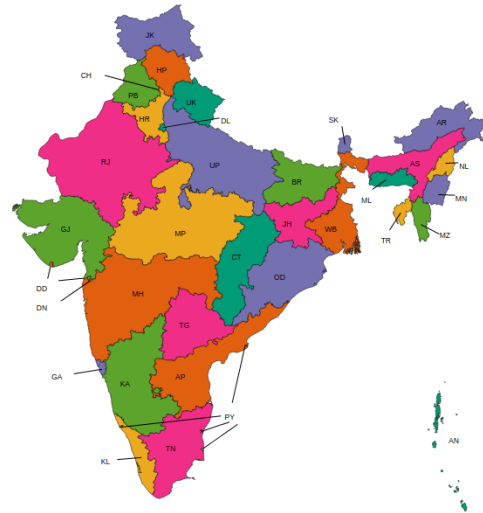

« Previous

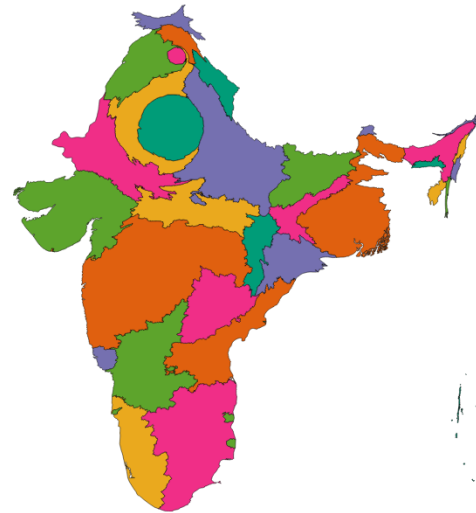

Next »

**(Cluster) Question 21 out of 43** On the other monitor, you can see a conventional map of India (left) and a GDP cartogram (right). Out of the states listed below, which has a GDP most similar to Uttar Pradesh (UP)?

- A. Delhi (DL)
- C. Rajasthan (RJ)

- B. Gujarat (GJ)
- D. Tamil Nadu (TN)

## Question 22

You have access to the infotips, parallel highlighting, and map switching features.

Hover over map regions to see more information.

Population (1960) Population (2010) Area

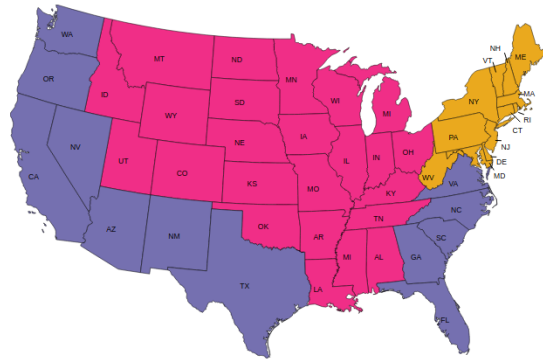

« Previous

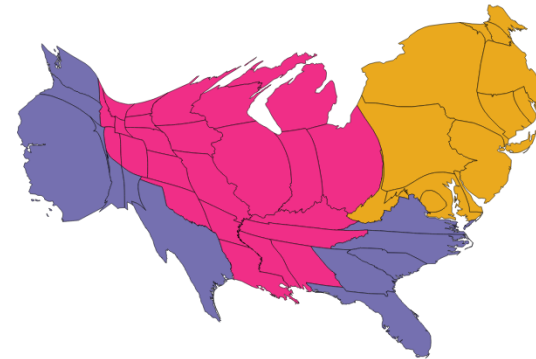

Next »

**(Summarize) Question 22 out of 43** On the other monitor, you can see a conventional map of the USA (left) and population cartograms for the years 1960 and 2010 (right). You may have to use the cartogram selector tab to view both cartograms. Three different regions are highlighted in yellow, purple and pink. What can you say about the change in population for each region from 1960 to 2010?

|                      |           |                            |              |
|----------------------|-----------|----------------------------|--------------|
| <b>Yellow Region</b> | A. Growth | B. Approximately No Change | C. Shrinking |
| <b>Pink Region</b>   | A. Growth | B. Approximately No Change | C. Shrinking |
| <b>Purple Region</b> | A. Growth | B. Approximately No Change | C. Shrinking |

### Question 23

You have access to the infotips, parallel highlighting, and map switching features.

Hover over map regions to see more information.

Population Land Area

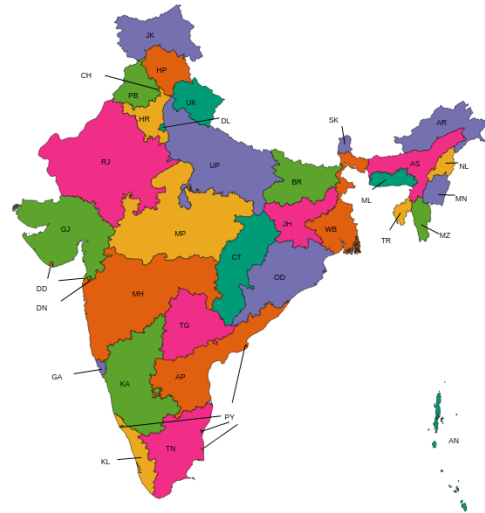

« Previous

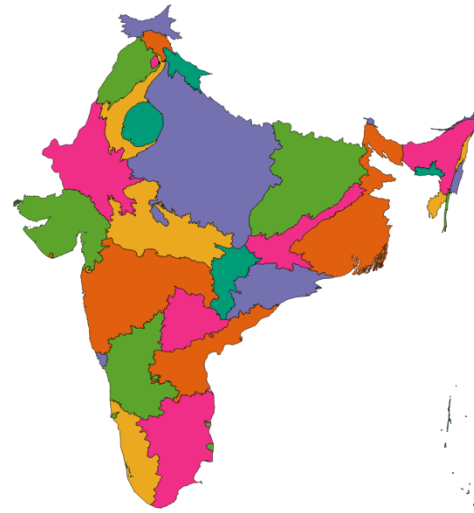

Next »

(Find adjacency) **Question 23 out of 43** On the other monitor, you can see a conventional map of India (left) and a population cartogram (right). What state(s) are **neighbours** of the state highlighted in red in the population cartogram below? **There may be more than one correct answer.**

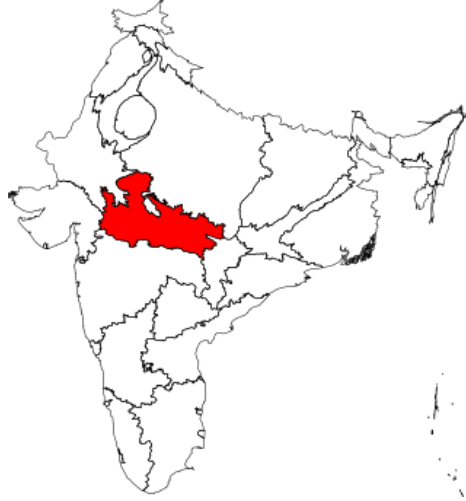

A. Delhi (DL)

B. Tamil Nadu (TN)

C. Uttar Pradesh (UP)

D. West Bengal (WB)



### Question 24

You have access to the infotips, parallel highlighting, and map switching features.

Hover over map regions to see more information.

Population Land Area

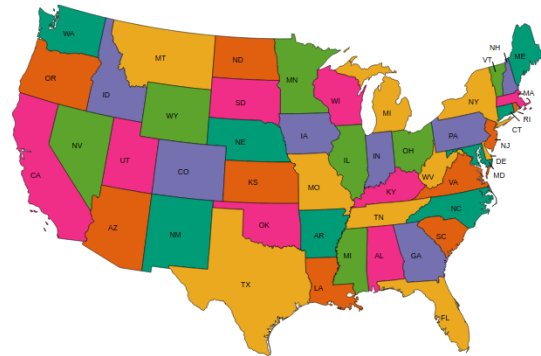

« Previous

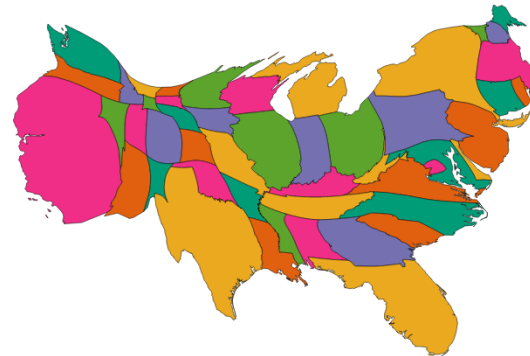

Next »

**(Recognize) Question 24 out of 43** On the other monitor, you can see a conventional map of the USA (left) and a population cartogram (right). What is the name of the state highlighted in red in the population cartogram below?

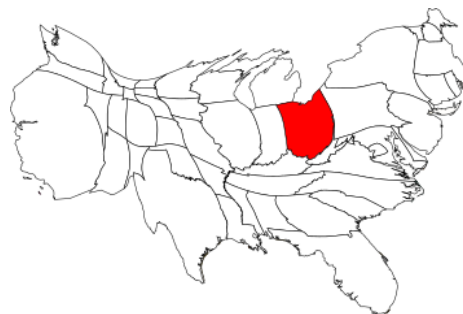

A. Florida (FL)

C. Ohio (OH)

B. Maine (ME)

D. California (CA)

### Question 25

You have access to the infotips, parallel highlighting, and map switching features.

Hover over map regions to see more information.

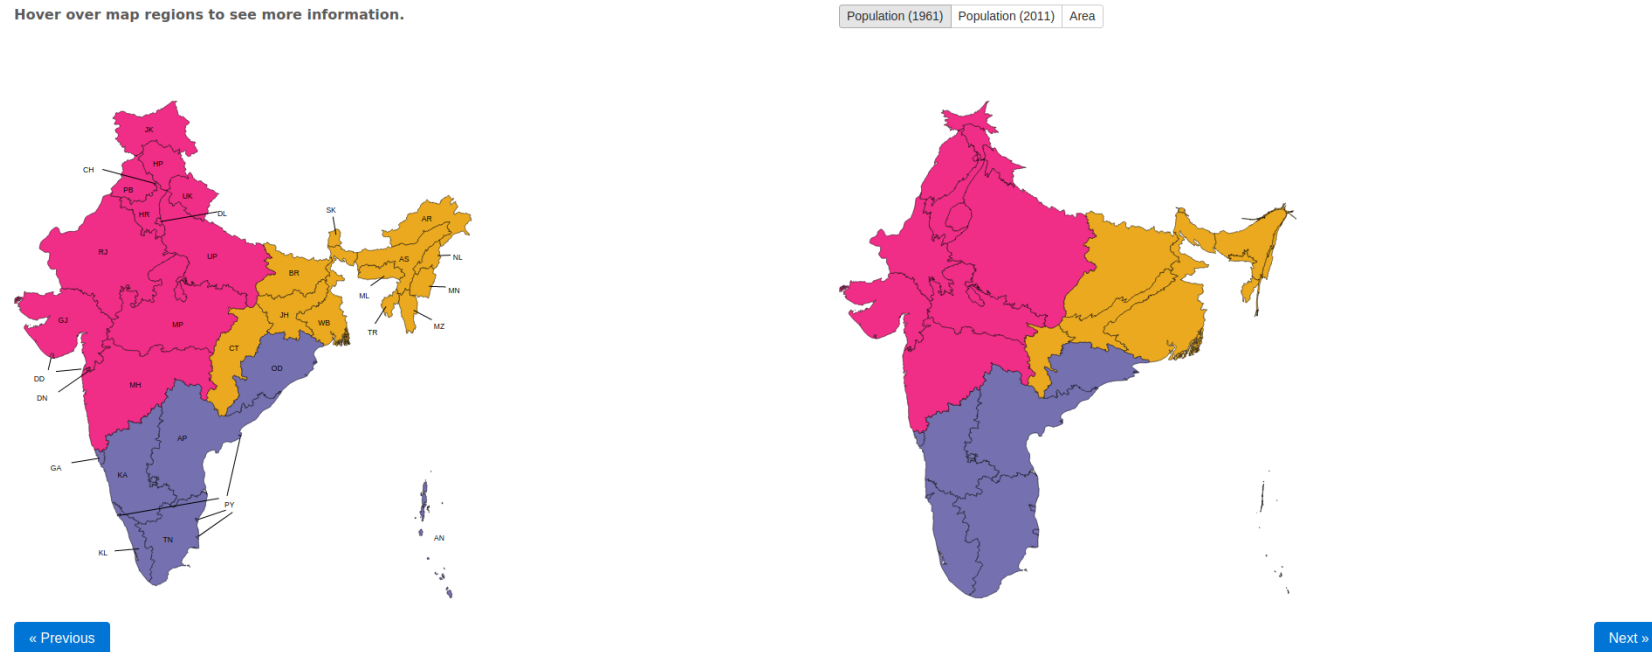

**(Summarize) Question 25 out of 43** On the other monitor, you can see a conventional map of India (left) and population cartograms for the years 1961 and 2011 (right). You may have to use the cartogram selector tab to view both cartograms. Three different regions are highlighted in yellow, purple and pink. What can you say about the change in population for each region from 1961 to 2011?

|                      |           |                            |              |
|----------------------|-----------|----------------------------|--------------|
| <b>Yellow Region</b> | A. Growth | B. Approximately No Change | C. Shrinking |
| <b>Pink Region</b>   | A. Growth | B. Approximately No Change | C. Shrinking |
| <b>Purple Region</b> | A. Growth | B. Approximately No Change | C. Shrinking |

### Question 26

You have access to the infotips, parallel highlighting, and map switching features.

Hover over map regions to see more information.

Population Land Area

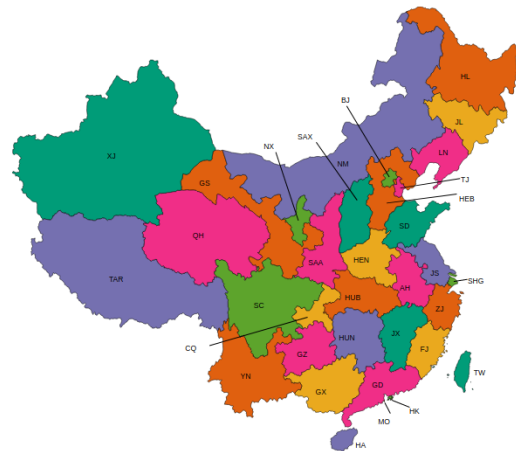

« Previous

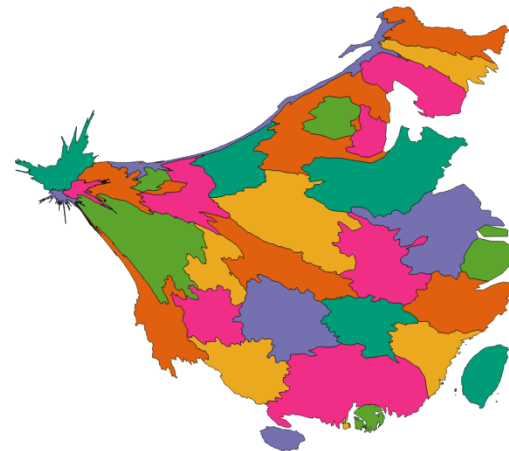

Next »

**(Recognize) Question 26 out of 43** On the other monitor, you can see a conventional map of Mainland China and Taiwan (left) and a population cartogram (right). What is the name of the region highlighted in red in the population cartogram below?

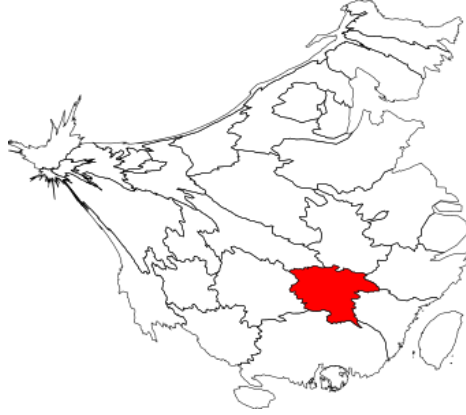

A. Hong Kong (HK)

B. Taiwan (TW)

C. Jiangxi (JX)

D. Beijing (BJ)

### Question 27

You have access to the infotips, parallel highlighting, and map switching features.

Hover over map regions to see more information.

Cows Population Land Area

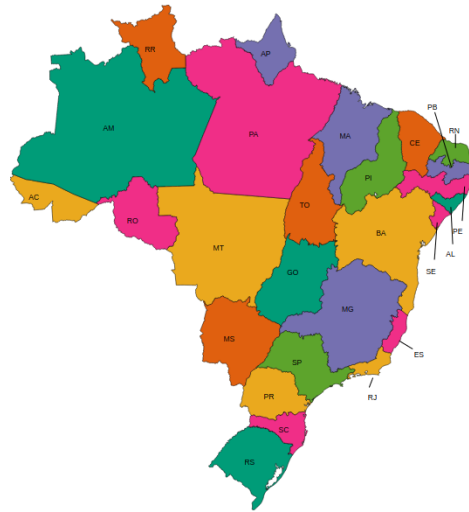

« Previous

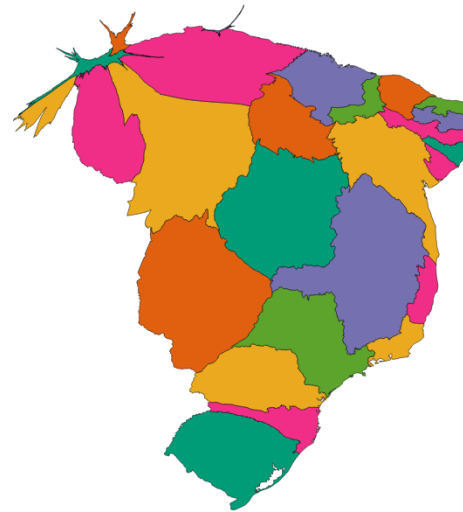

Next »

(Find top-k) Question 27 out of 43 On the other monitor, you can see a conventional map of Brazil (left) and a cattle population cartogram (right). Which state of Brazil has the highest cattle population?

- A. Mato Grosso (MG)
- C. Acre (AC)

- B. Amazonas (AM)
- D. Para (PA)

### Question 28

You have access to the infotips, parallel highlighting, and map switching features.

Hover over map regions to see more information.

Electoral Votes Population Land Area

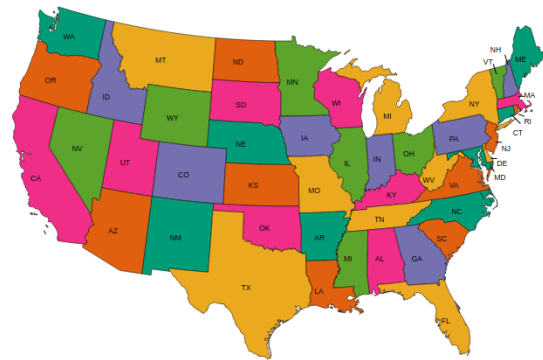

« Previous

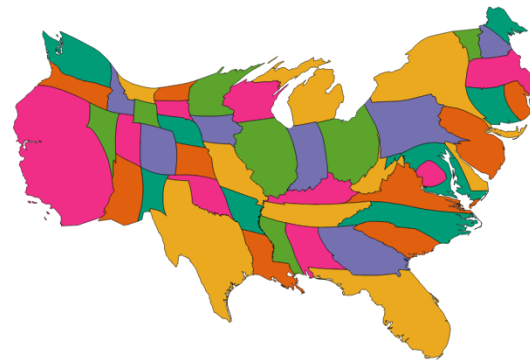

Next »

(Detect change) **Question 28 out of 43** On the other monitor, you can see a conventional map of the USA (left), an electoral vote cartogram (right). You may have to use the cartogram selector tab to view both cartograms. Is the area of California (CA) in the **electoral vote cartogram**

- higher than,
- approximately equal to or
- lower than

its area in the **population cartogram**?

A. Higher

B. Approximately equal

C. Lower

### Question 29

You have access to the infotips, parallel highlighting, and map switching features.

Hover over map regions to see more information.

Population Land Area

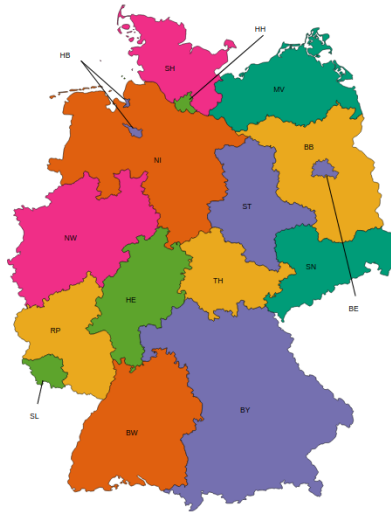

« Previous

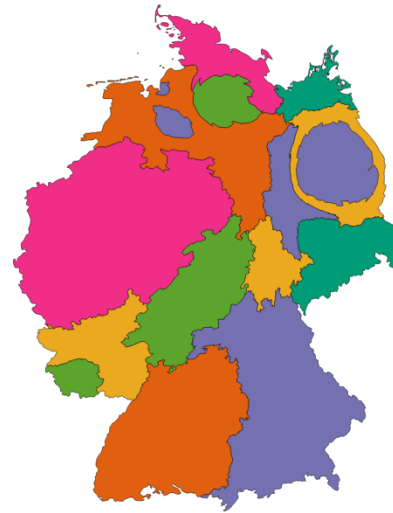

Next »

**(Cluster) Question 29 out of 43** On the other monitor, you can see a conventional map of Germany (left) and a population cartogram (right). Out of the states listed below, which has a population most similar to Sachsen (SN)?

- A. Berlin (BE)
- C. Thuringen (TH)

- B. Bremen (HB)
- D. Rheinland-Pfalz (RP)



### Question 30

You have access to the infotips, parallel highlighting, and map switching features.

Hover over map regions to see more information.

GDP Population Land Area

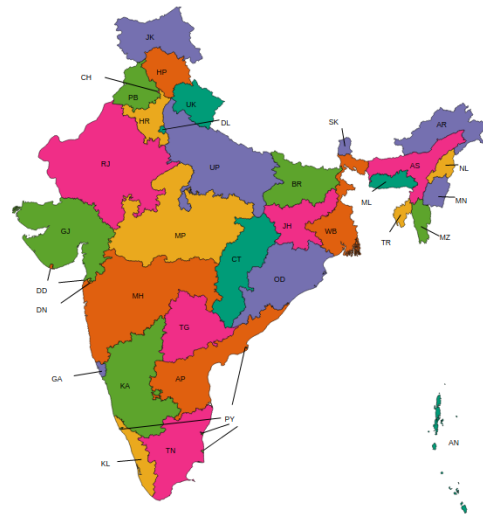

« Previous

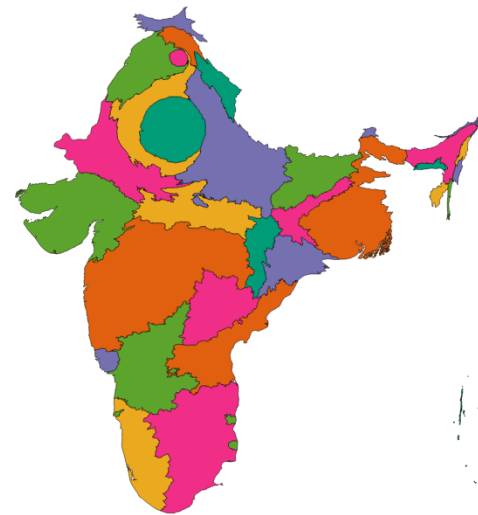

Next »

**(Compare) Question 30 out of 43** On the other monitor, you can see a conventional map of India (left) and a GDP cartogram (right). Is the GDP of Jharkhand (JH)

- higher than,
- approximately equal to or
- lower than

the GDP of Odisha (OD)?

A. Higher

C. Lower

B. Approximately equal

### Question 31

You have access to the infotips, parallel highlighting, and map switching features.

Hover over map regions to see more information.

Electoral Votes Population Land Area

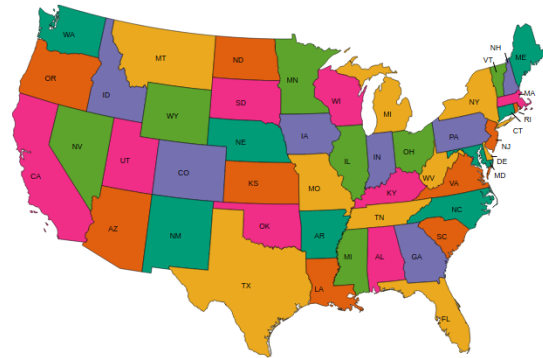

« Previous

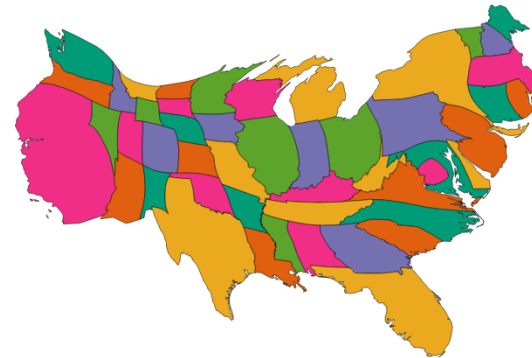

Next »

**(Filter) Question 31 out of 43** On the other monitor, you can see a conventional map of the USA (left) and an electoral vote cartogram (right). Out of the states listed below, which one(s) have a number of electoral votes higher than New York (NY)? **There may be more than one correct answer.**

A. Maine (ME)

B. California (CA)

C. Ohio (OH)

D. Texas (TX)

### Question 32

You have access to the infotips, parallel highlighting, and map switching features.

Hover over map regions to see more information.

GDP Population Land Area

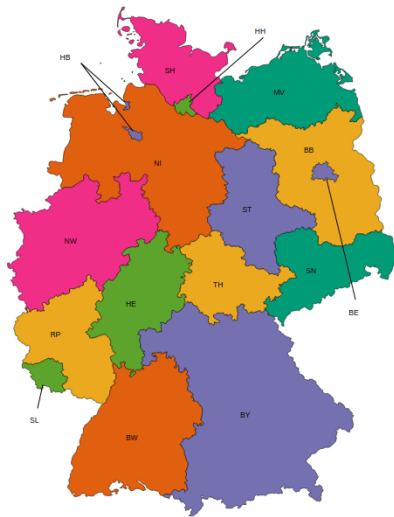

« Previous

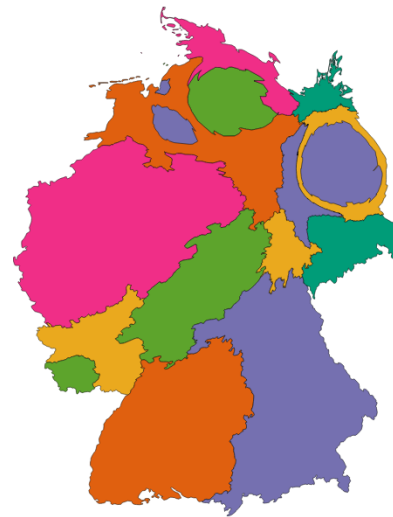

Next »

**(Detect change) Question 32 out of 43** On the other monitor, you can see a conventional map of Germany (left), a GDP cartogram and a population cartogram (right). You may have to use the cartogram selector tab to view both cartograms. Is the area of Hamburg (HH) in the **GDP cartogram**

- higher than,
- approximately equal to or
- lower than

its area in the **population cartogram**?

A. Higher

C. Lower

B. Approximately equal

### Question 33

You have access to the infotips, parallel highlighting, and map switching features.

Hover over map regions to see more information.

GDP Population Land Area

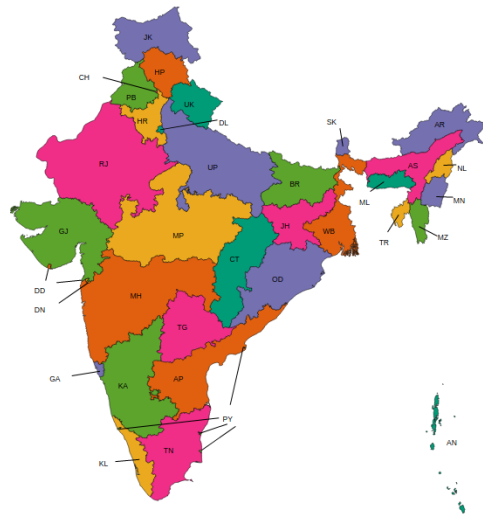

« Previous

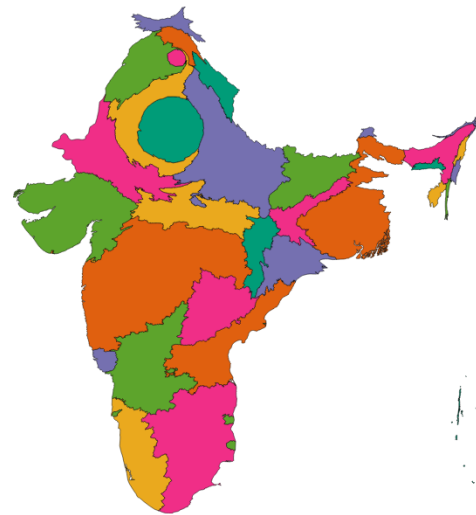

Next »

**(Find top-k) Question 33 out of 43** On the other monitor, you can see a conventional map of India (left) and a GDP cartogram (right). Which state of India has the highest GDP?

- A. Maharashtra (MH)
- C. Uttar Pradesh (UP)

- B. Tamil Nadu (TN)
- D. Rajasthan (RJ)

### Question 34

You have access to the infotips, parallel highlighting, and map switching features.

Hover over map regions to see more information.

Population (2000) Population (2030) Area

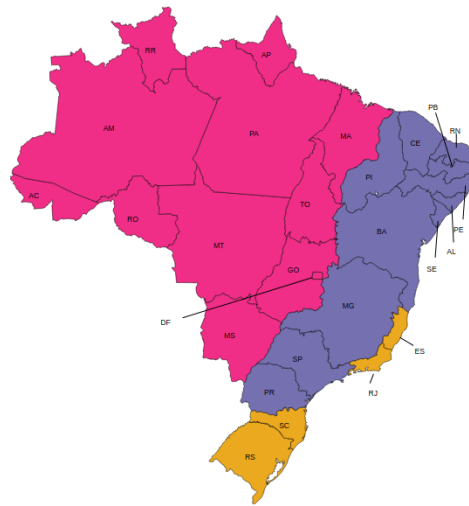

« Previous

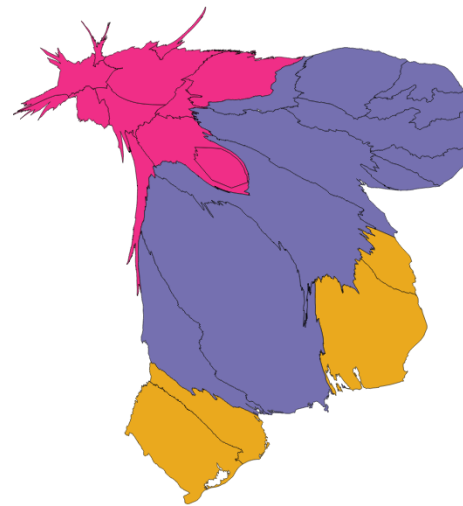

Next »

**(Summarize) Question 34 out of 43** On the other monitor, you can see a conventional map of Brazil (left) and population cartograms for the years 2000 and 2030 (projected population, right). You may have to use the cartogram selector tab to view both cartograms. Three different regions are highlighted in yellow, purple and pink. What can you say about the projected change in population for each region from 2000 to 2030?

|                      |           |                            |              |
|----------------------|-----------|----------------------------|--------------|
| <b>Yellow Region</b> | A. Growth | B. Approximately No Change | C. Shrinking |
| <b>Pink Region</b>   | A. Growth | B. Approximately No Change | C. Shrinking |
| <b>Purple Region</b> | A. Growth | B. Approximately No Change | C. Shrinking |

### Question 35

You have access to the infotips, parallel highlighting, and map switching features.

Hover over map regions to see more information.

GDP Population Land Area

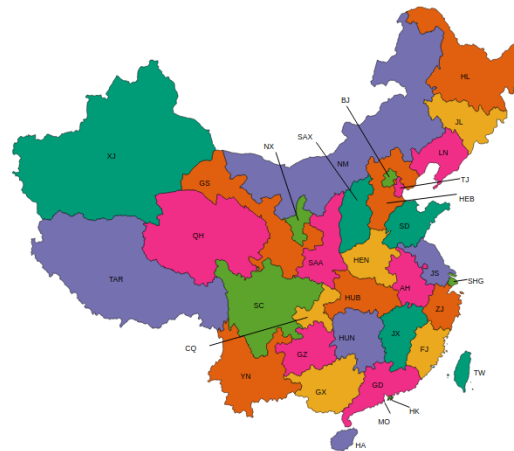

« Previous

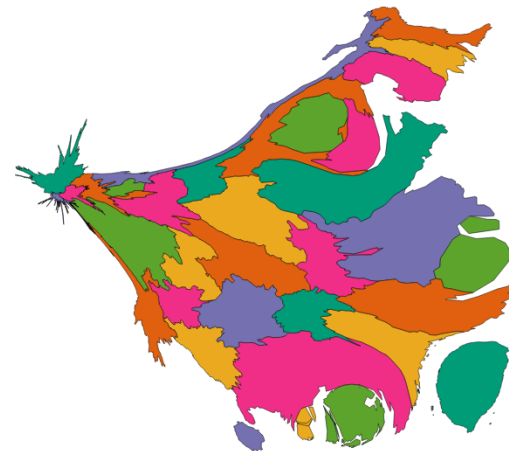

Next »

**(Filter) Question 35 out of 43** On the other monitor, you can see a conventional map of Mainland China and Taiwan (left) and a GDP cartogram (right). Out of the regions listed below, which one(s) have a GDP higher than Hong Kong (HK)? **There may be more than one correct answer.**

- A. Xinjiang (XJ)
- C. Heilongjiang (HL)

- B. Jiangsu (JS)
- D. Shandong (SD)



### Question 36

You have access to the infotips, parallel highlighting, and map switching features.

Hover over map regions to see more information.

Population Land Area

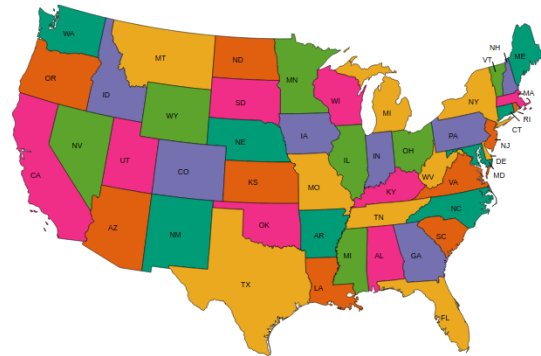

« Previous

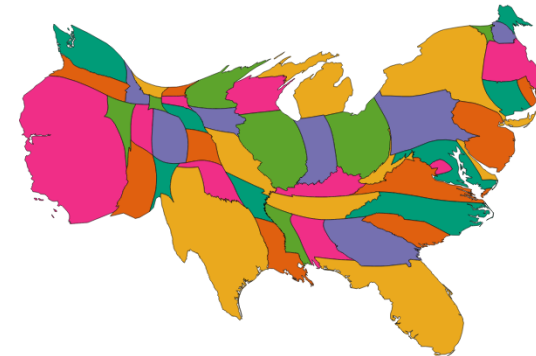

Next »

(Find adjacency) **Question 36 out of 43** On the other map, you can see a conventional map of the USA (left) and a population cartogram (right). What state(s) are **neighbours** of the state highlighted in red in the population cartogram below? **There may be more than one correct answer.**

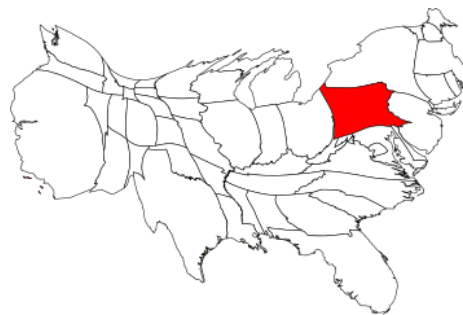

A. Maine (ME)

C. New Jersey (NJ)

B. Louisiana (LA)

D. New York (NY)

### Question 37

You have access to the infotips, parallel highlighting, and map switching features.

Hover over map regions to see more information.

Population Land Area

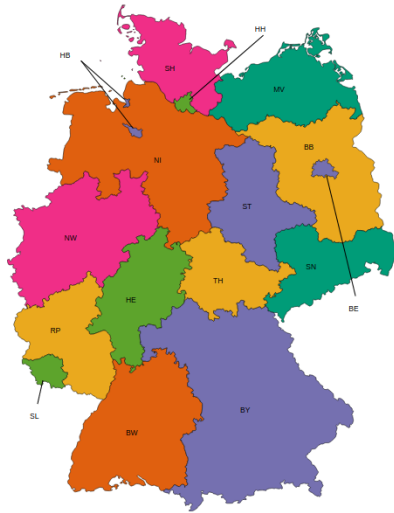

« Previous

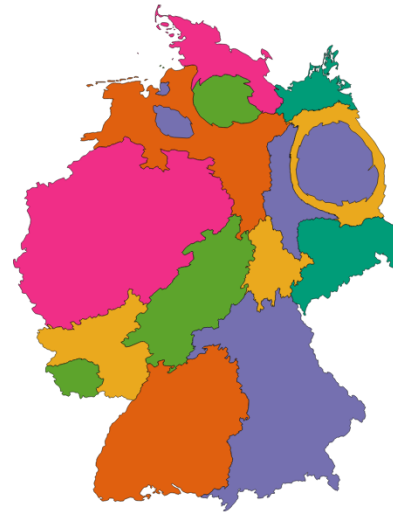

Next »

**(Recognize) Question 37 out of 43** On the other monitor, you can see a conventional map of Germany (left) and a population cartogram (right). What is the name of the state highlighted in red in the population cartogram below?

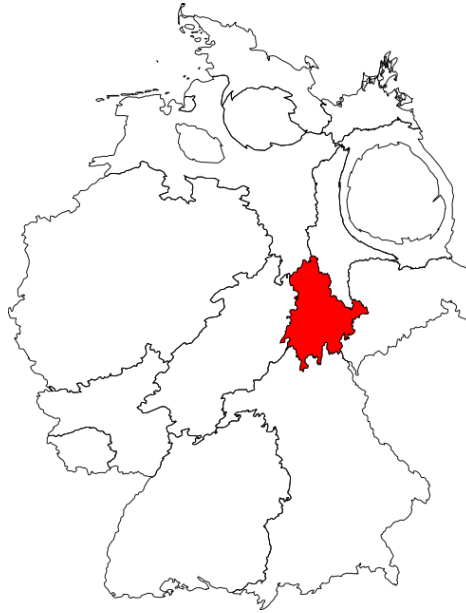

A. Saarland (SL)

C. Thuringen (TH)

B. Bayern (BE)

D. Bremen (HB)

### Question 38

You have access to the infotips, parallel highlighting, and map switching features.

Hover over map regions to see more information.

Population Land Area

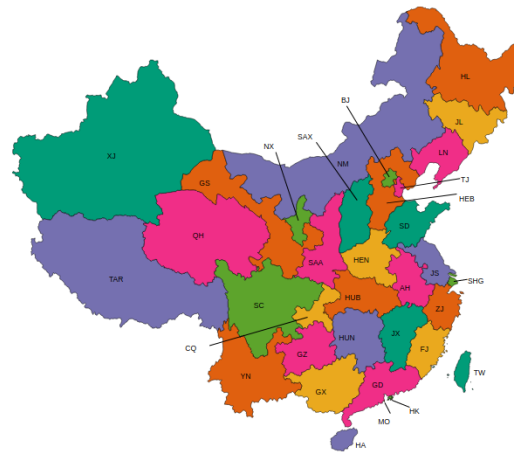

« Previous

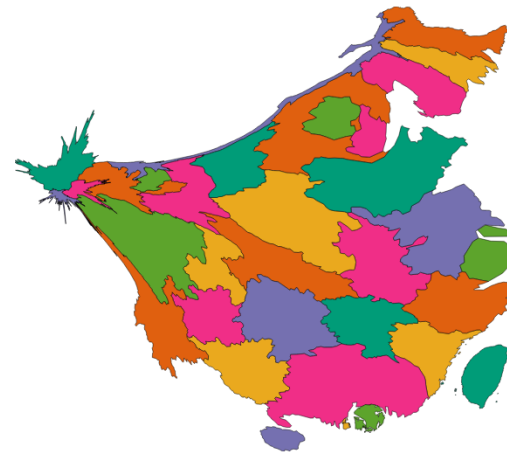

Next »

**(Find adjacency) Question 38 out of 43** On the other monitor, you can see a conventional map of Mainland China and Taiwan (left) and a population cartogram (right). What region(s) are neighbors of the region highlighted in red in the population cartogram below? There may be more than one correct answer.

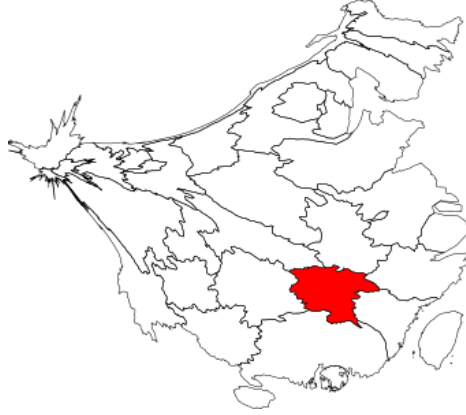

A. Hong Kong (HK)

B. Guangdong (GD)

C. Shandong (SD)

D. Beijing (BJ)

### Question 39

You have access to the infotips, parallel highlighting, and map switching features.

Hover over map regions to see more information.

GDP Population Land Area

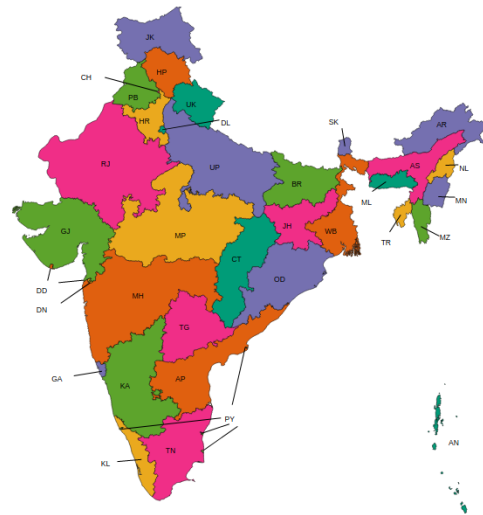

« Previous

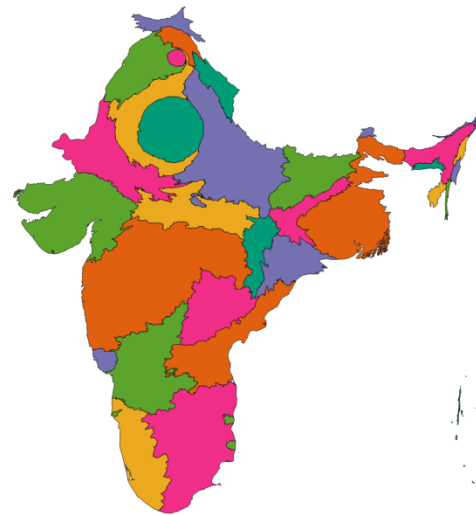

Next »

**(Detect change) Question 39 out of 43** On the other monitor, you can see a conventional map of India (left), a GDP cartogram and a population cartogram (right). Is the area of Odisha (OD) on the **GDP cartogram**

- higher than,
- approximately equal to or
- lower than

its area on the **population cartogram**?

A. Higher

C. Lower

B. Approximately equal



#### Question 40

You have access to the infotips, parallel highlighting, and map switching features.

Hover over map regions to see more information.

Cows Population Land Area

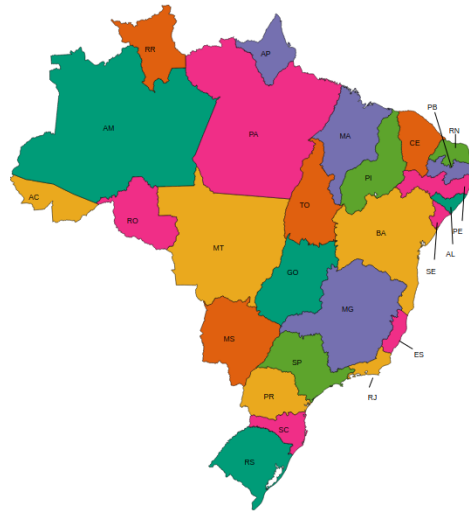

« Previous

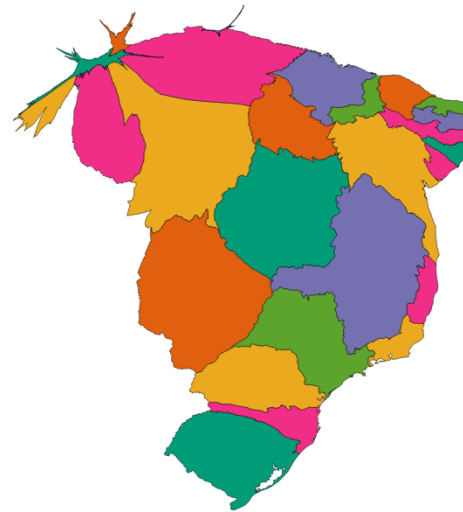

**(Filter) Question 40 out of 43** On the other monitor, you can see a conventional map of Brazil (left) and a cattle population cartogram (right). Out of the states listed below, which one(s) have a cattle population higher than Parana (PR)? **There may be more than one correct answer.**

- A. Mato Grosso do Sul (MS)
- C. Para (PA)

- B. Amazonas (AM)
- D. Sao Paulo (SP)

(Attitude Test) Question 41 out of 43

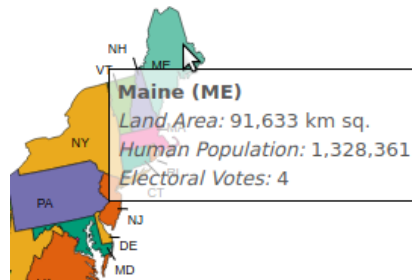

For each pair of words below, select the score that corresponds most closely with your view of the **infotip interactive feature** (i.e. the textbox in the upper left that appears when you hover over a region).

|                                    |   |   |   |   |   |                            |
|------------------------------------|---|---|---|---|---|----------------------------|
| Difficult to Use                   | 1 | 2 | 3 | 4 | 5 | Easy to Use                |
| Does not form immediate impression | 1 | 2 | 3 | 4 | 5 | Forms immediate impression |
| Conventional                       | 1 | 2 | 3 | 4 | 5 | Innovative                 |
| Redundant                          | 1 | 2 | 3 | 4 | 5 | Informative                |
| Hindering                          | 1 | 2 | 3 | 4 | 5 | Helpful                    |
| Boring                             | 1 | 2 | 3 | 4 | 5 | Entertaining               |
| Ugly                               | 1 | 2 | 3 | 4 | 5 | Elegant                    |

(Attitude Test) Question 42 out of 43

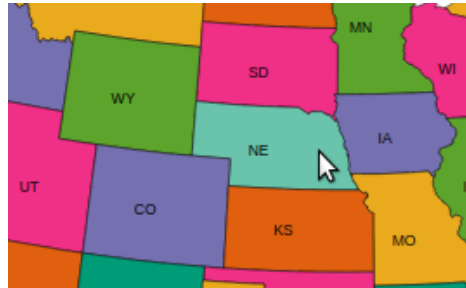

For each pair of words below, select the score that corresponds most closely with your view of the **parallel highlighting interactive feature**.

|                                    |   |   |   |   |   |                            |
|------------------------------------|---|---|---|---|---|----------------------------|
| Difficult to Use                   | 1 | 2 | 3 | 4 | 5 | Easy to Use                |
| Does not form immediate impression | 1 | 2 | 3 | 4 | 5 | Forms immediate impression |
| Conventional                       | 1 | 2 | 3 | 4 | 5 | Innovative                 |
| Redundant                          | 1 | 2 | 3 | 4 | 5 | Informative                |
| Hindering                          | 1 | 2 | 3 | 4 | 5 | Helpful                    |
| Boring                             | 1 | 2 | 3 | 4 | 5 | Entertaining               |
| Ugly                               | 1 | 2 | 3 | 4 | 5 | Elegant                    |

(Attitude Test) Question 43 out of 43

|                 |                  |           |
|-----------------|------------------|-----------|
| Electoral Votes | Human Population | Land Area |
|-----------------|------------------|-----------|

For each pair of words below, select the score that corresponds most closely with your view of the **map switching interactive feature**.

|                                    |   |   |   |   |   |                            |
|------------------------------------|---|---|---|---|---|----------------------------|
| Difficult to Use                   | 1 | 2 | 3 | 4 | 5 | Easy to Use                |
| Does not form immediate impression | 1 | 2 | 3 | 4 | 5 | Forms immediate impression |
| Conventional                       | 1 | 2 | 3 | 4 | 5 | Innovative                 |
| Redundant                          | 1 | 2 | 3 | 4 | 5 | Informative                |
| Hindering                          | 1 | 2 | 3 | 4 | 5 | Helpful                    |
| Boring                             | 1 | 2 | 3 | 4 | 5 | Entertaining               |
| Ugly                               | 1 | 2 | 3 | 4 | 5 | Elegant                    |
